# Supplementary material for: Adjoint Method in PDE-based Image Compression
Source: arXiv:2302.02665 source file (2024-10-10)
Supplement: Supplementary file 1 [file appendix00.tex]

\section{Some Asymptotic Developments} \label{app:calculus}

In this appendix, we state and prove some asymptotic developments for the quantities introduced in Proposition \ref{prop:solution-unhomo}. \\

\begin{lemma} \label{lem:asymptotic-1} For $\varepsilon$ small enough, we have for all $\varepsilon\leq r\leq R$,
    \[ A_{0,0}^\text{p}(r) - A_{\varepsilon,0}^\text{p}(r) = \frac{\alpha^{-1}}{2}h_0(x_0)\,\varepsilon^2\ln{\varepsilon} + o(\varepsilon^2\ln{\varepsilon}), \]
    and
    \[ B_{0,0}^\text{p}(r) - B_{\varepsilon,0}^\text{p}(r) = \frac{\alpha^{-1}}{2} h_0(x_0)\,\varepsilon^2 + o(\varepsilon^2). \]
\end{lemma}
\begin{proof} We have,
    \begin{align*}
        A_{0,0}^\text{p}(r) - A_{\varepsilon,0}^\text{p}(r) & = -\alpha^{-1}\int_0^\varepsilon s\,K_0(\alpha^{-1/2}\, s) h_0(s)\ ds.
    \end{align*}
    For $\varepsilon$ small enough, we have,
    \begin{align*}
        A_{0,0}^\text{p}(r) - A_{\varepsilon,0}^\text{p}(r) & = -\alpha^{-1}\,h_0(x_0) \int_0^\varepsilon s\,K_0(\alpha^{-1/2}\, s)\ ds + O(1) \int_0^\varepsilon s^2\,K_0(\alpha^{-1/2}\, s)\ ds.
    \end{align*}
    Moreover, we have \cite{Oldham2009},
    \begin{align*}
         \int_0^\varepsilon s\,K_0(\alpha^{-1/2}\, s)\ ds & = \alpha \left(1 - \alpha^{-1/2}\varepsilon K_1(\alpha^{-1/2}\,\varepsilon)\right) \\
         & = \alpha \left( 1 - \alpha^{-1/2}\varepsilon \left( \frac{1}{\alpha^{-1/2}\varepsilon} + \frac{\alpha^{-1/2}}{2} \varepsilon\ln{\Big(\frac{\alpha^{-1/2}}{2}\varepsilon\Big)} + o(\varepsilon\ln{\varepsilon}) \right) \right) \\
         & = -\frac{1}{2} \varepsilon^2\ln{\varepsilon} + o(\varepsilon^2\ln{\varepsilon}).
    \end{align*}
    We got the result. Same for $B_{\varepsilon,0}^\text{p} - B_{0,0}^\text{p}$.
\end{proof}

\begin{lemma} \label{lem:asymptotic-2} For $\varepsilon$ small enough, we have,
    \[ A_{0,0} - A_{\varepsilon,0} = -A_{0,0} \frac{K_0(\alpha^{-1/2}R)}{I_0(\alpha^{-1/2}\, R)} \frac{-1}{\ln{\varepsilon}} + o\left(\frac{-1}{\ln{\varepsilon}}\right), \]
    and
    \[ B_{\varepsilon, 0} = -A_{0,0}\frac{-1}{\ln{\varepsilon}} + o\left(\frac{-1}{\ln{\varepsilon}}\right), \]
    where $A_{0,0}$ is defined in Proposition \ref{prop:solution-unhomo}.
\end{lemma}

\begin{proof}
    We have,
    $$ A_{0,0} - A_{\varepsilon, 0} = \frac{K_0(\alpha^{-1/2}\varepsilon) \Theta_\varepsilon + I_0(\alpha^{-1/2}\varepsilon) K_0(\alpha^{-1/2}R) A_{0,0}}{I_0(\alpha^{-1/2}\varepsilon)K_0(\alpha^{-1/2}R) - K_0(\alpha^{-1/2}\varepsilon)I_0(\alpha^{-1/2}R)}, $$
    and,
    $$ B_{\varepsilon, 0} = \frac{I_0(\alpha^{-1/2}\varepsilon) \Theta_\varepsilon + I_0(\alpha^{-1/2}\varepsilon) I_0(\alpha^{-1/2}R) A_{0, 0}}{I_0(\alpha^{-1/2}\varepsilon)K_0(\alpha^{-1/2}R) - K_0(\alpha^{-1/2}\varepsilon)I_0(\alpha^{-1/2}R)}, $$
    where, $$ \Theta_\varepsilon := \big(A_{0, 0}^\text{p}(R) - A_{\varepsilon, 0}^\text{p}(R)\big)I_0(\alpha^{-1/2}R) + \big(B_{0, 0}^\text{p}(R) - B_{\varepsilon, 0}^\text{p}(R) \big)K_0(\alpha^{-1/2}R). $$
    We use that, \cite{Abramowitz1972}, (we set $\Gamma := \gamma-\ln{2} + \ln{\alpha^{-1/2}}$),
    \[ K_0(\alpha^{-1/2} \varepsilon) = -(\Gamma + \ln{\varepsilon}) I_0(\alpha^{-1/2} \varepsilon) + \varepsilon r_1(\varepsilon), \]
    and we get,
    $$ A_{0,0} - A_{\varepsilon, 0} = \frac{-1}{\ln{\varepsilon}}\frac{ -K_0(\alpha^{-1/2}R) A_{0,0} + \big( \Gamma + \ln{\varepsilon} + \varepsilon r_3(\varepsilon) \big) \Theta_\varepsilon}{I_0(\alpha^{-1/2}R) + \frac{C}{\ln{\varepsilon}} + \varepsilon r_2(\varepsilon)} , $$
    and,
    $$ B_{\varepsilon, 0} = \frac{-1}{\ln{\varepsilon}} \frac{- I_0(\alpha^{-1/2}R) A_{0, 0} -\Theta_\varepsilon }{I_0(\alpha^{-1/2}R) + \frac{C}{\ln{\varepsilon}} + \varepsilon r_2(\varepsilon)}, $$
    where, $$ C := K_0(\alpha^{-1/2}R) + \Gamma I_0(\alpha^{-1/2}R). $$
    Moreover, using Lemma \ref{lem:asymptotic-1}, we have,
    $$ \Theta_\varepsilon = \frac{\alpha^{-1}}{2} h_0(x_0) I_0(\alpha^{-1/2}R) \varepsilon^2\ln{\varepsilon} + \varepsilon^2\ln{\varepsilon} r_3(\varepsilon). $$
    We have the results.
\end{proof}

\begin{lemma} For all $n$ in $\N$, we have when $\varepsilon$ is small enough, 
    $$ B_{0,n}^\text{p}(r) - B_{\varepsilon,n}^\text{p}(r) = \frac{2^{-n}\alpha^{-n/2}}{n!(n+2)} \varepsilon^{n+2} + o(\varepsilon^{n+2}), $$
    for all $\varepsilon \leq r \leq R$.
\end{lemma}
\begin{proof} We have,
    \begin{align*}
        B_{0,n}^\text{p}(r) - B_{\varepsilon,n}^\text{p}(r) & = \alpha^{-1}\int_0^\varepsilon s\,I_n(\alpha^{-1/2}\, s) h_n(s)\ ds.
    \end{align*}
    For $\varepsilon$ small enough, we have,
    \begin{align*}
        B_{0,n}^\text{p}(r) - B_{\varepsilon,n}^\text{p}(r) & = \alpha^{-1}\,h_n(x_0) \int_0^\varepsilon s\,I_n(\alpha^{-1/2}\, s)\ ds + O(1) \int_0^\varepsilon s^2\,I_n(\alpha^{-1/2}\, s)\ ds.
    \end{align*}
    Moreover, we have \cite{Oldham2009},
    \begin{align*}
         \int_0^\varepsilon s\,I_n(\alpha^{-1/2}\, s)\ ds & = \frac{2^{-n}\alpha^{-n/2}}{n!}\int_0^\varepsilon s^{n+1}\ ds + o(\varepsilon^{n+2}) = \frac{2^{-n}\alpha^{-n/2}}{n!(n+2)} \varepsilon^{n+2} + o(\varepsilon^{n+2}).
    \end{align*}    
\end{proof}
