# Supplementary material for: Adjoint Method in PDE-based Image Compression
Source: arXiv:2302.02665 source file (2024-10-10)
Supplement: Supplementary file 2 [file appendix02.tex]

\section{Étude du Problème Extérieur}

Dans cette section nous allons donner des estimations de la solution du problème extérieur avec les normes définies dans l'Appendix A. Pour $\psi$ dans $H^{1/2}(\partial B_1)$, on définit le problème extérieur comme : 

\[ \left \{ \begin{array}{cc}
    -\alpha\Delta v_\omega + v_\omega = 0, & \text{dans}\ \R^2\setminus B(0,1), \\
    v_\omega = \psi, & \text{sur}\ \partial B(0,1), \\
    v_\omega = 0, & \text{à}\ \infty.
\end{array} \right .\]

Alors \\

\begin{proposition}
    Pour $y$ dans $\R^2\setminus\bar{B_1}$, 
    \[ v_\omega(y) = \int_{\partial B_1} E(y-x) p(x)\ d\sigma(x), \]
    
    où $E$ est la solution fondamentale (radiale) dans $\R^2\setminus\{0\}$ donnée par
    
    \[ E(y) := \frac{1}{2\pi} K_0\left(\frac{1}{\sqrt{\alpha}}|y|\right), \]
    
    et $p$ solution dans $H^{-1/2}(\partial B_1)$ de
    
    \[ \int_{\partial B_1} E(y-x) p(x)\ d\sigma(x) = \psi(y),\ \forall y\in\partial B_1. \]
\end{proposition}
\begin{proof}
    On dérive et on utilise \cite{Oldham2009} : $K_0'(z) = -K_1(z)$ et $K_1'(z) = -K_0(z) - \frac{1}{z}K_1(z)$.
\end{proof}
% \begin{note}
%     Si $\psi$ est une constante, alors 
    
%     \[ v_\omega(y) = \frac{\psi}{K_0\left(\alpha^{-1/2}\right)} K_0\left(\alpha^{-1/2}|y|\right). \]
% \end{note}

% Pour $|y|$ grand, on fait Taylor et avec \cite{Oldham2009}, on a 
    
% \[ E(y-x) = \sqrt{\frac{\pi}{2\sqrt{\alpha}}}e^{-|y|/\sqrt{\alpha}}|y|^{-1/2} + O\left(e^{-|y|/\sqrt{\alpha}}|y|^{-3/2}\right). \]

% D'où

% \[ v_\omega(y) =  \sqrt{\frac{\pi}{2\sqrt{\alpha}}}\frac{e^{-|y|/\sqrt{\alpha}}}{\sqrt{|y|}}\int_{\partial B_1} p(x)\ d\sigma(x) + O\left(\frac{e^{-|y|}}{\sqrt{|y|}}\right). \]

% En faisant un développement limite de l'exponentielle à l'infini, on obtient

% \[ v_\omega(y) =  \sqrt{\frac{\pi}{2\sqrt{\alpha}}} |y|^{-1/2} \int_{\partial B_1} p(x)\ d\sigma(x) + O\left(|y|^{-3/2}\right). \]

% On pose 

% \[ V(y) := \sqrt{\frac{\pi}{2\sqrt{\alpha}}}|y|^{-1/2}\int_{\partial B_1} p(x)\ d\sigma(x), \]
% \[ W(y) := O\left(|y|^{-3/2}\right). \]

% ------------------------------------------------------------

\begin{proposition} Pour $|y|$ suffisamment grand, on a

    \[ v_\omega(y) = \tilde{V}(y) + \tilde{W}(y), \]
    et
    \[ \nabla v_\omega(y) = \nabla \tilde{V}(y) + \nabla \tilde{W}(y), \]
    
    avec 
    
    \begin{align*}
        & \tilde{V}(y) = \frac{1}{2\pi} K_0\left(\frac{|y|}{\sqrt{\alpha}}\right) \int_{\partial B_1}  p(x)\ d\sigma(x), \\
        & \tilde{W}(y) = O\left(K_0\left(\frac{|y|}{\sqrt{\alpha}}\right)\right), \\
        & \nabla \tilde{V}(y) = -\frac{1}{2\pi} K_1\left(\frac{|y|}{\sqrt{\alpha}}\right) |y|^{-1} y \int_{\partial B_1} p(x)\ d\sigma(x), \\
        & \nabla \tilde{W}(y) = O\left( K_1\left(\frac{|y|}{\sqrt{\alpha}}\right) |y|^{-1} y\right).
    \end{align*}
\end{proposition}
\begin{proof}
    Pour $|y|$ grand, on fait Taylor,
    
    \begin{align*}
        v_\omega(y) & = \int_{\partial B_1} E\big(|y|\big) p(x)\ d\sigma(x) - \int_{\partial B_1} \nabla_y E\big(|y|\big)\cdot x\, p(x)\ d\sigma(x) + o(1) \\
        & = \frac{1}{2\pi} K_0\left(\frac{|y|}{\sqrt{\alpha}}\right) \int_{\partial B_1}  p(x)\ d\sigma(x) + \frac{1}{2\pi} K_1\left(\frac{|y|}{\sqrt{\alpha}}\right) |y|^{-1} \int_{\partial B_1} y \cdot x\, p(x)\ d\sigma(x) + o(1).
    \end{align*}

    On pose 
    
    \begin{align*}
        & \tilde{V}(y) = \frac{1}{2\pi} K_0\left(\frac{|y|}{\sqrt{\alpha}}\right) \int_{\partial B_1}  p(x)\ d\sigma(x), \\
        & \tilde{W}(y) = \frac{1}{2\pi} K_1\left(\frac{|y|}{\sqrt{\alpha}}\right) |y|^{-1} \int_{\partial B_1} y \cdot x\, p(x)\ d\sigma(x) + o(1) = O\left(K_0\left(\frac{|y|}{\sqrt{\alpha}}\right)\right).
    \end{align*}

    Et on a donc 
    
    \[ v_\omega(y) = \tilde{V}(y) + \tilde{W}(y) \]
    et
    \[ \nabla \tilde{V}(y) = -\frac{1}{2\pi} K_1\left(\frac{|y|}{\sqrt{\alpha}}\right) |y|^{-1} y \int_{\partial B_1} p(x)\ d\sigma(x). \]
    
    De plus, 
    
    \begin{align*}
        \nabla v_\omega(y) & = \nabla \tilde{V}(y) + \nabla \tilde{W}(y) \\
        & = -\frac{1}{2\pi} y \int_{\partial B_1} K_1\left(\frac{|y-x|}{\sqrt{\alpha}}\right) |y-x|^{-1} p(x)\ d\sigma(x) \\
        & = -\frac{1}{2\pi} K_1\left(\frac{|y|}{\sqrt{\alpha}}\right) |y|^{-1} y \int_{\partial B_1}  p(x)\ d\sigma(x) + O\left( K_1\left(\frac{|y|}{\sqrt{\alpha}}\right) |y|^{-1} y\right).
    \end{align*}
    
    D'où 
    
    \[ \nabla \tilde{W}(y) = O\left( K_1\left(\frac{|y|}{\sqrt{\alpha}}\right) |y|^{-1} y\right). \]
\end{proof}

\begin{proposition} Pour $|y|$ suffisamment grand, on a

    \[ v_\omega(y) = V(y) + W(y), \]
    et
    \[ \nabla v_\omega(y) = \nabla V(y) + \nabla W(y), \]
    
    avec 
    
    \begin{align*}
        & V(y) := \sqrt{\frac{1}{8\pi\sqrt{\alpha}}}|y|^{-1/2}e^{-|y|/\sqrt{\alpha}}\int_{\partial B_1} p(x)\ d\sigma(x), \\
        & W(y) := O\big(|y|^{-3/2}e^{-|y|/\sqrt{\alpha}}\big), \\
        & \nabla V(y) = - \sqrt{\frac{1}{8\pi\sqrt{\alpha}}} e^{\left(-\frac{|y|}{\sqrt{\alpha}}\right)} |y|^{-1} \left( \frac{1}{\sqrt{\alpha} \sqrt{|y|}} + \frac{1}{2 \, |y|^{\frac{3}{2}}} \right) y \int_{\partial B_1} p(x)\ d\sigma(x), \\
        & \nabla W(y) = O\big(|y|^{-5/2}e^{-|y|/\sqrt{\alpha}}\big)y.
    \end{align*}
\end{proposition}
\begin{proof}
    On utilise \cite{Oldham2009}, pour $x$ assez grand
    
    \[ K_\nu(x) = \sqrt{\frac{\pi}{2}}\,x^{-1/2}\,e^{-x} + O(x^{-3/2}\,e^{-x}). \]
\end{proof}

\begin{proposition} Pour $|y|$ suffisamment grand, il existe $C_1,C_2,C_3$ et $C_4$ ne dépendant que de $\alpha$ telles que
    \begin{align*}
        |V(y)| & \leq C_1\, |y|^{-1/2}e^{-|y|/\sqrt{\alpha}}\, \|\psi\|, \\
        |\nabla V(y)| & \leq C_2\,|y|^{-1/2}e^{-|y|/\sqrt{\alpha}} \, \|\psi\|, \\
        |W(y)| & \leq C_3\, |y|^{-3/2}\, \|\psi\|, \\
        |\nabla W(y)| & \leq C_4\, |y|^{-3/2}\, \|\psi\|.
    \end{align*}
\end{proposition}
\begin{proof}
    Puisque $K_0$ est positive et décroissante, on a pour $(x,z)\in(\partial B_1)^2$,
    
    \[ E(x-z) \geq \frac{1}{2\pi}K_0(2\alpha^{-1/2}) \Leftrightarrow \frac{2\pi}{K_0(2\alpha^{-1/2})}E(x-z) \geq 1. \]
    
    D'où pour $z\in\partial B_1$,
    
    \[ \left|\int_{\partial B_1} p(x) d\sigma(x)\right| \leq \frac{2\pi}{K_0(2\alpha^{-1/2})}\left|\int_{\partial B_1} E(x-z) p(x)\ d\sigma(x)\right| = \frac{2\pi}{K_0(2\alpha^{-1/2})} |\psi(z)|. \]
    
    En passant au carré et en intégrant l'inégalité sur $\partial B_1$ par rapport à $z$,
    
    \[ \left|\int_{\partial B_1} p(x) d\sigma(x)\right|^2 \leq \frac{2\pi}{K_0(2\alpha^{-1/2})^2}\int_{\partial B_1} |\psi(z)|^2\ d\sigma(z). \]
    
    Soit $u=\psi$ sur $\partial B_1$. Alors
    
    \[ \left|\int_{\partial B_1} p(x) d\sigma(x)\right|^2 \leq \frac{2\pi}{K_0(2\alpha^{-1/2})^2}\int_{B_1\setminus B_{1/2}} |u(z)|^2\ dz, \]
    
    ceci étant vrai pour tout $u$ on a
    
    \[ \left|\int_{\partial B_1} p(x) d\sigma(x)\right|^2 \leq \frac{2\pi}{K_0(2\alpha^{-1/2})^2}\|\psi\|_{1/2,\partial B_1}^2. \]
    
    \textbullet ~ \textbf{Montrons (1) :} \\

    \[ |V(y)| = \sqrt{\frac{1}{8\pi\sqrt{\alpha}}}|y|^{-1/2}e^{-|y|/\sqrt{\alpha}} \left| \int_{\partial B_1} p(x)\ d\sigma(x)\right|. \]
    
    \textbullet ~ \textbf{Montrons (2) :} \\

    % \[ \nabla V(y) = - \sqrt{\frac{1}{8\pi\sqrt{\alpha}}} e^{\left(-\frac{|y|}{\sqrt{\alpha}}\right)} |y|^{-1} \left( \frac{1}{\sqrt{\alpha} \sqrt{|y|}} + \frac{1}{2 \, |y|^{\frac{3}{2}}} \right) y \int_{\partial B_1} p(x)\ d\sigma(x) \]
    
    % d'où 
    
    \[ |\nabla V(y)| = \sqrt{\frac{1}{8\pi\sqrt{\alpha}}} e^{\left(-\frac{|y|}{\sqrt{\alpha}}\right)} \left( \frac{1}{\sqrt{\alpha} \sqrt{|y|}} + \frac{1}{2 \, |y|^{\frac{3}{2}}} \right) \left|\int_{\partial B_1} p(x)\ d\sigma(x)\right|. \]

    \textbullet ~ \textbf{Montrons (3) :} \\
    
    Pour être plus précis, lorsqu'on a fait Taylor on avait 
    
    \[ W(y) = O\big(|y|^{-3/2}e^{-|y|/\sqrt{\alpha}}\big)\int_{\partial B_1} p(x) d\sigma(x). \]
    
    Par définition du grand $O$, il existe $K>0$ et $R_0>1$ tels que, pour tout $|y|>R_0$, on a
    
    \[ |W(y)| \leq K |y|^{-3/2}e^{-|y|/\sqrt{\alpha}} \left|\int_{\partial B_1} p(x) d\sigma(x)\right|. \]
    
    \textbullet ~ \textbf{Montrons (4) :} Pareil que (3) \\
    
    % On a que
    
    % \[ \nabla v_\omega(y) = \nabla V(y) + \nabla W(y) \]
    
    % En faisant Taylor à l'ordre $2$ et en utilisant
    
    % \[ \nabla_y E\big(|y|\big) = -\frac{1}{2\pi} K_1\left(\frac{|y|}{\sqrt{\alpha}}\right) |y|^{-1} y, \]
    
    % on obtient
    
    % \[ \nabla v_\omega(y) = \frac{1}{2\pi} K_0\left(\frac{|y|}{\sqrt{\alpha}}\right) \int_{\partial B_1} p(x)\ d\sigma(x) + \frac{1}{2\pi} K_1\left(\frac{|y|}{\sqrt{\alpha}}\right) |y|^{-1} \int_{\partial B_1} y\cdot x\, p(x)\ d\sigma(x) \] \[ + O\left(K_1\left(\frac{|y|}{\sqrt{\alpha}}\right) |y|^{-1} \right)\int_{\partial B_1} y\cdot x\, p(x)\ d\sigma(x). \]
    
    % D'où
    
    % \[ \nabla W(y) = \nabla v_\omega(y) - \nabla V(y) = O\left(K_1\left(\frac{|y|}{\sqrt{\alpha}}\right) |y|^{-1} y\right) = O\big(|y|^{-7/2}e^{-|y|/\sqrt{\alpha}}\big)y \]
\end{proof}

Avec les estimations de la proposition précédente, les deux propositions suivantes sont évidentes. \\

\begin{proposition} Pour $|y|$ suffisamment grand, il existe $C_1,C_2,C_3,C_4,C_5,C_6,C_7$ et $C_8$ ne dépendant que de $\alpha$ et de $R$, telles que, pour $\varepsilon$ suffisamment petit,

    \begin{align*}
        \|V\|_{0,B_{R/\varepsilon}\setminus B_1} & \leq C_1\, \|\psi\|_{1/2,\partial B_1}, \\
        |V|_{1,B_{R/\varepsilon}\setminus B_1} & \leq C_2\, \|\psi\|_{1/2,\partial B_1}, \\
        \|W\|_{0,B_{R/\varepsilon}\setminus B_1} & \leq C_3\, \|\psi\|_{1/2,\partial B_1}, \\
        |W|_{1,B_{R/\varepsilon}\setminus B_1} & \leq C_4\, \, \|\psi\|_{1/2,\partial B_1}, \\
        \|V\|_{0,B_{R/\varepsilon}\setminus B_{R/(2\varepsilon)}} & \leq C_5\, e^{-R/(\varepsilon\sqrt{\alpha})}\, \|\psi\|_{1/2,\partial B_1}, \\
        |V|_{1,B_{R/\varepsilon}\setminus B_{R/(2\varepsilon)}} & \leq C_6\, e^{-R/(\varepsilon\sqrt{\alpha})}\, \|\psi\|_{1/2,\partial B_1}, \\
        \|W\|_{0,B_{R/\varepsilon}\setminus B_{R/(2\varepsilon)}} & \leq C_7\, \varepsilon^{1/2} \,\|\psi\|_{1/2,\partial B_1}, \\
        |W|_{1,B_{R/\varepsilon}\setminus B_{R/(2\varepsilon)}} & \leq C_8\, \varepsilon^{1/2}\, \|\psi\|_{1/2,\partial B_1}.
    \end{align*}
\end{proposition}

et aussi \\

\begin{proposition} Pour $|y|$ suffisamment grand, il existe $C_1,C_2,C_3,C_4,C_5$ et $C_6$ ne dépendant que de $\alpha$ telles que, pour $\varepsilon$ suffisamment petit,

    \begin{align*}
        \|v_\omega\|_{0,B_{R/\varepsilon}\setminus B_1} & \leq C_1\, \|\psi\|_{1/2,\partial B_1}, \\
        |v_\omega|_{1,B_{R/\varepsilon}\setminus B_1} & \leq C_2\, \|\psi\|_{1/2,\partial B_1}, \\
        \|v_\omega\|_{1,B_{R/\varepsilon}\setminus B_1} & \leq C_3\, \|\psi\|_{1/2,\partial B_1}, \\
        \|v_\omega\|_{0,B_{R/\varepsilon}\setminus B_{R/(2\varepsilon)}} & \leq C_4\,\varepsilon^{1/2}\, \|\psi\|_{1/2,\partial B_1}, \\
        |v_\omega|_{1,B_{R/\varepsilon}\setminus B_{R/(2\varepsilon)}} & \leq C_5\, \varepsilon^{1/2}\, \|\psi\|_{1/2,\partial B_1}, \\
        \|v_\omega\|_{1,B_{R/\varepsilon}\setminus B_{R/(2\varepsilon)}} & \leq C_6\,\varepsilon^{1/2}\, \|\psi\|_{1/2,\partial B_1}.
    \end{align*}
\end{proposition}
