# Supplementary material for: Adjoint Method in PDE-based Image Compression
Source: arXiv:2302.02665 source file (2024-10-10)
Supplement: Supplementary file 3 [file appendix02b.tex]

\section{Problème Extérieur}

\subsection{Trou normalisé}

Pour $\psi$ dans $H^{1/2}(\partial B_1)$,

\[ \left \{ \begin{array}{cc}
    -\alpha\Delta v_\omega + v_\omega = 0, & \text{dans}\ \R^2\setminus B(0,1), \\
    v_\omega = \psi, & \text{sur}\ \partial B(0,1), \\
    v_\omega = 0, & \text{à}\ \infty.
\end{array} \right .\]

\begin{proposition}
    Pour $y$ dans $\R^2\setminus\bar{B_1}$, 
    \[ v_\omega(y) = \int_{\partial B_1} E(y-x) p(x)\ d\sigma(x), \]
    
    où $E$ est la solution fondamentale (radiale) dans $\R^2\setminus\{0\}$ donnée par
    
    \[ E(y) := \frac{1}{2\pi} K_0\left(\frac{1}{\sqrt{\alpha}}|y|\right), \]
    
    et $p$ solution dans $H^{-1/2}(\partial B_1)$ de
    
    \[ \int_{\partial B_1} E(y-x) p(x)\ d\sigma(x) = \psi(y),\ \forall y\in\partial B_1. \]
\end{proposition}
\begin{proof}
    On dérive et on utilise \cite{Oldham2009} :
    
    \[ K_0'(z) = -K_1(z), \]
    \[ K_1'(z) = -K_0(z) - \frac{1}{z}K_1(z). \]
\end{proof}

Pour $|y|$ grand, on fait Taylor et avec \cite{Oldham2009}, on a 
    
\[ E(y-x) = \sqrt{\frac{\pi}{2\sqrt{\alpha}}}\frac{e^{-|y|/\sqrt{\alpha}}}{\sqrt{|y|}} + O\left(\frac{e^{-|y|}}{\sqrt{|y|}}\right). \]

D'où

\[ v_\omega(y) =  \sqrt{\frac{\pi}{2\sqrt{\alpha}}}\frac{e^{-|y|/\sqrt{\alpha}}}{\sqrt{|y|}}\int_{\partial B_1} p(x)\ d\sigma(x) + O\left(\frac{e^{-|y|}}{\sqrt{|y|}}\right). \]

On pose 

\[ V(y) := \sqrt{\frac{\pi}{2\sqrt{\alpha}}}\frac{e^{-|y|/\sqrt{\alpha}}}{\sqrt{|y|}}\int_{\partial B_1} p(x)\ d\sigma(x), \]
\[ W(y) := O\left(\frac{e^{-|y|}}{\sqrt{|y|}}\right). \]

\begin{proposition} Pour tout $y\in \R^2\setminus B_1$, il existe $C_1,C_2,C_3$ et $C_4$ ne dépendant que de $\alpha$ telles que
    \[ |V(y)| \leq C_1\, |y|^{-1/2} e^{-|y|/\sqrt{\alpha}}\, \|\psi\|_{1/2,\partial B_1}, \]
    \[ **|\nabla V(y)| \leq C_2\, |y|^{-1/2}e^{-|y|/\sqrt{\alpha}}\, \|\psi\|_{1/2,\partial B_1}, \]
    \[ |W(y)| \leq C_3\, |y|^{-1/2}e^{-|y|}\, \|\psi\|_{1/2,\partial B_1}, \]
    \[ ->|\nabla W(y)| \leq C_4\, e^{-|y|}\, \|\psi\|_{1/2,\partial B_1}. \]
\end{proposition}
\begin{proof}
    \textbullet ~ \textbf{Montrons (1) :} \\
    
    Puisque $K_0$ est positive et décroissante, on a pour $(x,z)\in(\partial B_1)^2$,
    
    \[ E(x-z) \geq \frac{1}{2\pi}K_0(2\alpha^{-1/2}) \Leftrightarrow \frac{2\pi}{K_0(2\alpha^{-1/2})}E(x-z) \geq 1. \]
    
    D'où pour $z\in\partial B_1$,
    
    \[ \left|\int_{\partial B_1} p(x) d\sigma(x)\right| \leq \frac{2\pi}{K_0(2\alpha^{-1/2})}\left|\int_{\partial B_1} E(x-z) p(x)\ d\sigma(x)\right| = \frac{2\pi}{K_0(2\alpha^{-1/2})} |\psi(z)|. \]
    
    En passant au carré et en intégrant l'inégalité sur $\partial B_1$ par rapport à $z$,
    
    \[ \left|\int_{\partial B_1} p(x) d\sigma(x)\right|^2 \leq \frac{2\pi}{K_0(2\alpha^{-1/2})^2}\int_{\partial B_1} |\psi(z)|^2\ d\sigma(z). \]
    
    Ainsi,
    
    \[ |V(y)|^2 = \left(\sqrt{\frac{\pi}{2\sqrt{\alpha}}}\frac{e^{-|y|/\sqrt{\alpha}}}{\sqrt{|y|}}\right)^2 \left|\int_{\partial B_1} p(x)\ d\sigma(x)\right|^2 \leq \frac{2\pi}{K_0(2\alpha^{-1/2})^2}\left(\sqrt{\frac{\pi}{2\sqrt{\alpha}}}\frac{e^{-|y|/\sqrt{\alpha}}}{\sqrt{|y|}}\right)^2\int_{\partial B_1} |\psi(z)|^2\ d\sigma(z). \]
    
    Soit $u=\psi$ sur $\partial B_1$. Alors
    
    \[ |V(y)|^2 \leq \frac{2\pi}{K_0(2\alpha^{-1/2})^2}\left(\sqrt{\frac{\pi}{2\sqrt{\alpha}}}\frac{e^{-|y|/\sqrt{\alpha}}}{\sqrt{|y|}}\right)^2\int_{B_1\setminus B_{1/2}} |u(z)|^2\ dz. \]
    
    Ceci étant vrai pour tout $u$ on a le résultat. \\
    
    \textbullet ~ \textbf{Montrons (2) :} \\

    \[ \partial_{y_i}V(y) = -\sqrt{\frac{\pi}{8\,\alpha^{3/2}}}\, \frac{ {\left(2 \, |y|  + \sqrt{\alpha} \right)} e^{\left(-\frac{|y|}{\sqrt{\alpha}}\right)}}{ |y|^{\frac{5}{2}}}\, \int_{\partial B_1} p(x)\ d\sigma(x)\, y_i,\ i=1,2, \]
    
    d'où 
    
    \[ |\nabla V(y)|^2 = \left(\big(\partial_{y_1} V(y)\big)^2 +  \big(\partial_{y_2} V(y)\big)^2\right) \left|\int_{\partial B_1} p(x) d\sigma(x)\right|^2 \]
    \[ = \frac{\pi}{8 \, \alpha^{\frac{3}{2}}}\frac{{\left(4 \, |y|^{2} + 4 \, \sqrt{\alpha} |y| + \alpha\right)} e^{\left(-\frac{2 \, |y|}{\sqrt{\alpha}}\right)}}{ |y|^{3}}  \left|\int_{\partial B_1} p(x) d\sigma(x)\right|^2 \]
    \[ = \frac{\pi}{4 \, \alpha^{\frac{3}{2}}} |y|^{-1} e^{-2|y|/\sqrt{\alpha}} \left|\int_{\partial B_1} p(x) d\sigma(x)\right|^2 + o\left(|y|^{-1} e^{-2|y|/\sqrt{\alpha}}\right). \]
    \[ \leq  C |y|^{-1} e^{-2|y|/\sqrt{\alpha}} \left|\int_{\partial B_1} p(x) d\sigma(x)\right|^2. \]
    
    En faisant la même chose que pour l'inégalité précédente, on a le résultat.
    
    \textbullet ~ \textbf{Montrons (3) :} \\
    
    Pour être plus précis, lorsqu'on a fait Taylor on avait 
    
    \[ W(y) = O\left(\frac{e^{-|y|}}{\sqrt{|y|}}\right)\int_{\partial B_1} p(x) d\sigma(x). \]
    
    Par définition du grand $O$, il existe $K>0$ et $R_0>1$ tels que, pour tout $|y|>R_0$, on a
    
    \[ |W(y)| \leq K \frac{e^{-|y|}}{\sqrt{|y|}}\left|\int_{\partial B_1} p(x) d\sigma(x)\right|. \]
    
    Avec le même raisonnement que pour les inégalités précédentes, on a le résultat. \\
    
    \textbullet ~ \textbf{Montrons (4) :} \\
    
    \[ \nabla v_\omega(y) = \nabla V(y) + \nabla W(y) \]
    
    \[ \int_{\partial B_1} \nabla_y E(y-x) p(x)\ d\sigma(x) = \nabla V(y) + \nabla W(y) \]
    
    \[ \frac{1}{2\pi}\int_{\partial B_1} \nabla_y K_0(|x-y|) p(x)\ d\sigma(x) = \nabla V(y) + \nabla W(y) \]
    
    \[ \frac{1}{2\pi}\int_{\partial B_1} \left( -\frac{K_1(|x-y|)}{|x-y|}y \right) p(x)\ d\sigma(x) = -\sqrt{\frac{\pi}{8\,\alpha^{3/2}}}\, \frac{ {\left(2 \, |y|  + \sqrt{\alpha} \right)} e^{\left(-\frac{|y|}{\sqrt{\alpha}}\right)}}{ |y|^{\frac{5}{2}}}\, \int_{\partial B_1} p(x)\ d\sigma(x)\, y + \nabla W(y). \]
    
    Een appliquant Taylor et \cite{Oldham2009} sur le membre de gauche pour $|y|$ grand,
    
    \[ \sqrt{\frac{\pi}{2\sqrt{\alpha}}}\frac{e^{-|y|/\sqrt{\alpha}}}{\sqrt{|y|}}y \int_{\partial B_1} p(x)\ d\sigma(x) + O\left(\frac{e^{-|y|/\sqrt{\alpha}}}{\sqrt{|y|}}\right)\int_{\partial B_1} p(x)\ d\sigma(x) = -\sqrt{\frac{\pi}{8\,\alpha^{3/2}}}\, \frac{ {\left(2 \, |y|  + \sqrt{\alpha} \right)} e^{-|y|/\sqrt{\alpha}}}{ |y|^{\frac{5}{2}}}\, \int_{\partial B_1} p(x)\ d\sigma(x)\, y \]\[ + \nabla W(y). \]
    
    D'où 
    
    \[ \nabla W(y) = \frac{\sqrt{2\pi}}{4}\frac{{2 |y|^{\frac{5}{2}} \sqrt{\frac{1}{\sqrt{\alpha}}} + 2 |y|^{\frac{3}{2}} \sqrt{\frac{1}{\alpha^{\frac{3}{2}}}} + \sqrt{\alpha} \sqrt{|y|} \sqrt{\frac{1}{\alpha^{\frac{3}{2}}}}} }{|y|^{3}} e^{-|y|/\sqrt{\alpha}}\, y\, \int_{\partial B_1} p(x)\ d\sigma(x) + O\left(\frac{e^{-|y|/\sqrt{\alpha}}}{\sqrt{|y|}}\right)\int_{\partial B_1} p(x)\ d\sigma(x) \]
    
    \[ |\nabla W(y)| = o\left(K_1(|y|)\right)\int_{\partial B_1} p(x)\ d\sigma(x). \]
    
    Avec le même raisonnement que pour les inégalités précédentes, on a le résultat.
\end{proof}

\begin{proposition} Pour tout $y\in \R^2\setminus B_1$, il existe $C_1,C_2,C_3$ et $C_4$ ne dépendant que de $\alpha$ telles que
    \[ \|V\|_{0,B_{R/\varepsilon}\setminus B_1} \leq C_1\, \left(e^{-2 /\sqrt{\alpha}}-e^{-2 R/(\sqrt{\alpha}\varepsilon)}\right)^{1/2}\, \|\psi\|_{1/2,\partial B_1}, \]
    
    \[ |V|_{1,B_{R/\varepsilon}\setminus B_1} \leq C_2\, \left(e^{-2/\sqrt{\alpha}} - \frac{\varepsilon}{R}e^{-2R/(\sqrt{\alpha}\varepsilon)}\right)^{1/2}\, \|\psi\|_{1/2,\partial B_1}, \]
    
    \[ \|W\|_{0,B_{R/\varepsilon}\setminus B_1} \leq C_3\, \left(e^{-2}-e^{-2 R/\varepsilon}\right)^{1/2}\, \|\psi\|_{1/2,\partial B_1}, \]
    
    \[ \|V\|_{0,B_{R/(2\varepsilon)}\setminus B_{R/\varepsilon}} \leq C_4\,\left(e^{-2R /(\sqrt{\alpha}\varepsilon)}-e^{- R/(\sqrt{\alpha}\varepsilon)}\right)^{1/2}\, \|\psi\|_{1/2,\partial B_1}, \]
    
    \[ |V|_{1,B_{R/(2\varepsilon)}\setminus B_{R/\varepsilon}} \leq C_5\, \left(e^{-2R/(\sqrt{\alpha}\varepsilon)} - \frac{2\varepsilon}{R}e^{-R/(\sqrt{\alpha}\varepsilon)}\right)^{1/2}\, \|\psi\|_{1/2,\partial B_1}, \]
    
    \[ \|W\|_{0,B_{R/(2\varepsilon)}\setminus B_{R/\varepsilon}} \leq C_6\, \left(e^{-2R/\varepsilon}-e^{-R/\varepsilon}\right)^{1/2}\, \|\psi\|_{1/2,\partial B_1}, \]
    
    \[ |W|_{1,B_{R/\varepsilon}\setminus B_1} \leq C_7, \]
    
    \[ |W|_{1,B_{R/(2\varepsilon)}\setminus B_{R/\varepsilon}} \leq C_8. \]
\end{proposition}
\begin{proof}
    \textbullet ~ \textbf{Montrons (1) :} \\
    
    \[ \|V\|_{0,B_{R/\varepsilon}\setminus B_1}^2 = \int_{B_{R/\varepsilon}\setminus B_1} |V(y)|^2\ dy \]
    \[ \leq C_1^2\,\|\psi\|_{1/2,\partial B_1}^2\, \int_{B_{R/\varepsilon}\setminus B_1}|y|^{-1} e^{-2|y|/\sqrt{\alpha}}\ dy. \]
    
    On passe en coordonnées polaires : 
    
    \[ \|V\|_{0,B_{R/\varepsilon}\setminus B_1}^2 \leq 2\pi C_1^2\,\|\psi\|_{1/2,\partial B_1}^2\, \int_1^{R/\varepsilon} e^{-2 r/\sqrt{\alpha}}\ dr \]
    \[ = \pi \sqrt{\alpha} C_1^2\,\|\psi\|_{1/2,\partial B_1}^2\, \left(e^{-2 /\sqrt{\alpha}}-e^{-2 R/(\sqrt{\alpha}\varepsilon)}\right). \]
    
    \textbullet ~ \textbf{Montrons (2) :} \\
    
    \[ |V|_{1,B_{R/\varepsilon}\setminus B_1}^2 = \int_{B_{R/\varepsilon}\setminus B_1} |\nabla V(y)|^2\ dy \]
    \[ \leq C_2^2\, \|\psi\|_{1/2,\partial B_1}^2\, \int_{B_{R/\varepsilon}} |y|^{-3}e^{-2|y|/\sqrt{\alpha}}\ dy. \]
    
    On passe en coordonnées polaires : 
    
    \[ |V|_{1,B_{R/\varepsilon}\setminus B_1}^2 \leq C_2^2\, \|\psi\|_{1/2,\partial B_1}^2\, \int_1^{R/\varepsilon} r^{-2}e^{-2r/\sqrt{\alpha}}\ dr \]
    \[ = C_2^2\, \|\psi\|_{1/2,\partial B_1}^2\, \left(\left[\frac{-1}{r}e^{-2r/\sqrt{\alpha}}\right]_1^{R/\varepsilon} - \frac{2}{\sqrt{\alpha}}\int_1^{R/\varepsilon} r^{-1}e^{-2r/\sqrt{\alpha}}\ dr \right) \]
    \[ \leq C_2^2\, \|\psi\|_{1/2,\partial B_1}^2\, \left[\frac{-1}{r}e^{-2r/\sqrt{\alpha}}\right]_1^{R/\varepsilon} \]
    \[ = C_2^2\, \|\psi\|_{1/2,\partial B_1}^2\, \left(e^{-2/\sqrt{\alpha}} - \frac{\varepsilon}{R}e^{-2R/(\sqrt{\alpha}\varepsilon)}\right). \]
    
    \textbullet ~ \textbf{Montrons (3) :} \\
    
    Pareil que (1).
    
    \textbullet ~ \textbf{Montrons (4) :} \\
    
    Pareil que (1).
    
    \textbullet ~ \textbf{Montrons (5) :} \\
    
    Pareil que (1).
\end{proof}

\subsection{Trou $\varepsilon$}

Pour $\psi_\varepsilon$ dans $H^{1/2}(\partial B_\varepsilon)$,

\[ \left \{ \begin{array}{cc}
    -\alpha\Delta v_{\omega_\varepsilon} + v_{\omega_\varepsilon} = 0, & \text{dans}\ \R^2\setminus B(0,\varepsilon), \\
    v_{\omega_\varepsilon} = \psi_\varepsilon, & \text{sur}\ \partial B(0,\varepsilon), \\
    v_{\omega_\varepsilon} = 0, & \text{à}\ \infty.
\end{array} \right .\]

\begin{proposition}
    
\end{proposition}
\begin{proof} Soit $y\in \R^2\setminus B_1$,
    \[ v_{\omega_\varepsilon}( \varepsilon y ) = v_\omega(y) \]
\end{proof}

\begin{proposition}
    Pour tout $y\in \R^2\setminus B_\varepsilon$, il existe $C_1,C_2,C_3$ et $C_4$ ne dépendant que de $\alpha$ telles que  
    
    \[ \|V\|_{0,B_{R/\varepsilon}\setminus B_1} \leq  \]
\end{proposition}
\begin{proof}
    
\end{proof}
