# Supplementary material for: Adjoint Method in PDE-based Image Compression
Source: arXiv:2302.02665 source file (2024-10-10)
Supplement: Supplementary file 4 [file appendix02c.tex]

\subsection{Exterior Problem}
\label{appendix:exterior-pb}

Now, we give estimates of the solution to the \textit{exterior} problem with the norms defined previously. For $\phi$ in $H^{1/2}(\partial B_1)$, we define the exterior problem as the following :
\[ \left \{ \begin{array}{cl}
    -\alpha\Delta v_\omega + v_\omega = 0, & \text{in}\ \R^2\setminus B_1, \\
    v_\omega = \phi, & \text{on}\ \partial B_1, \\
    v_\omega = 0, & \text{at}\ \infty.
\end{array} \right .\]
The aim of this appendix is to prove the following proposition : \\

\begin{proposition} There exists $C_1,C_2,C_3,C_4,C_5$ and $C_6$ only dependant on $\alpha$ such that, for $\varepsilon$ small enough,
    \begin{align*}
        \|v_\omega\|_{0,B_{R/\varepsilon}\setminus B_1} & \leq C_1\, \|\phi\|_{1/2,\partial B_1}, \\
        |v_\omega|_{1,B_{R/\varepsilon}\setminus B_1} & \leq C_2\, \|\phi\|_{1/2,\partial B_1}, \\
        \|v_\omega\|_{1,B_{R/\varepsilon}\setminus B_1} & \leq C_3\, \|\phi\|_{1/2,\partial B_1}, \\
        \|v_\omega\|_{0,B_{R/\varepsilon}\setminus B_{R/(2\varepsilon)}} & \leq C_4\,e^{-R/(2\varepsilon\sqrt{\alpha})} \,\|\phi\|_{1/2,\partial B_1}, \\
        |v_\omega|_{1,B_{R/\varepsilon}\setminus B_{R/(2\varepsilon)}} & \leq C_5\,e^{-R/(2\varepsilon\sqrt{\alpha})} \,\|\phi\|_{1/2,\partial B_1}, \\
        \|v_\omega\|_{1,B_{R/\varepsilon}\setminus B_{R/(2\varepsilon)}} & \leq C_6\,e^{-R/(2\varepsilon\sqrt{\alpha})} \,\|\phi\|_{1/2,\partial B_1}.
    \end{align*}
    \label{prop:exterior-pb-estimates}
\end{proposition}

The proposition above can be derived easily from the results bellow : \\

\begin{proposition}
    For $y$ in $\R^2\setminus\overline{B_1}$, we have
    \[ v_\omega(y) = \int_{\partial B_1} E(y-x) p(x)\ d\sigma(x), \]
    where $E$ is the fundamental solution (radial) in $\R^2\setminus\{0\}$ given by
    \[ E(y) := \frac{1}{2\pi} K_0\left(\frac{1}{\sqrt{\alpha}}|y|\right), \]
    where $K_0$ is the modified Bessel function of the second kind \cite{Oldham2009} and $p$ is the solution in $H^{-1/2}(\partial B_1)$ of
    \[ \int_{\partial B_1} E(y-x) p(x)\ d\sigma(x) = \phi(y),\ \forall y\in\partial B_1. \]
\end{proposition}
\begin{proof}
    We differentiate and we use \cite{Oldham2009} : $K_0'(z) = -K_1(z)$ and $K_1'(z) = -K_0(z) - \frac{1}{z}K_1(z)$.
\end{proof}

\begin{proposition} For $|y|$ large enough, it exists $C_1$ and $C_2$, only dependant on $\alpha$, such that,
    \begin{align*}
        |v_\omega(y)| & \leq C_1\, |y|^{-1/2}e^{-|y|/\sqrt{\alpha}}\, \|\phi\|_{1/2,\partial B_1}, \\
        |\nabla v_\omega(y)| & \leq C_2\, |y|^{-1/2}e^{-|y|/\sqrt{\alpha}}\, \|\phi\|_{1/2,\partial B_1}.
    \end{align*}
\end{proposition}
\begin{proof}
    Since $K_0$ is a positive and decreasing function, we have for $(x,z)\in(\partial B_1)^2$,
    \[ E(x-z) \geq \frac{1}{2\pi}K_0(2\alpha^{-1/2}) \Leftrightarrow \frac{2\pi}{K_0(2\alpha^{-1/2})}E(x-z) \geq 1. \]
    Then, for $z\in\partial B_1$,
    \[ \left|\int_{\partial B_1} p(x) d\sigma(x)\right| \leq \frac{2\pi}{K_0(2\alpha^{-1/2})}\left|\int_{\partial B_1} E(x-z) p(x)\ d\sigma(x)\right| = \frac{2\pi}{K_0(2\alpha^{-1/2})} |\phi(z)|. \]
    We integrate on $\partial B_1$ with respect to $z$ the square of the previous inequality and get,
    \[ \left|\int_{\partial B_1} p(x) d\sigma(x)\right|^2 \leq \frac{2\pi}{K_0(2\alpha^{-1/2})^2}\int_{\partial B_1} |\phi(z)|^2\ d\sigma(z). \]
    Let $u=\phi$ on $\partial B_1$. Then,
    \[ \left|\int_{\partial B_1} p(x) d\sigma(x)\right|^2 \leq \frac{2\pi}{K_0(2\alpha^{-1/2})^2}\int_{B_1\setminus B_{1/2}} |u(z)|^2\ dz, \]
    this been true for every $u$, we take the $\sup$,
    \[ \left|\int_{\partial B_1} p(x) d\sigma(x)\right|^2 \leq \frac{2\pi}{K_0(2\alpha^{-1/2})^2}\|\phi\|_{1/2,\partial B_1}^2. \]
    
    With \cite{Oldham2009}, we have for $z$ big enough,
    \[ K_0(z) = O(z^{-1/2}e^{-z}), \]
    thus, there exists $C>0$, such that, for $|y|$ large enough,
    \[ |E(x-y)| \leq C\,|x-y|^{-1/2}e^{-|x-y|/\sqrt{\alpha}}. \]
    Moreover, for $|y|$ large enough,
    \[ |x-y|^{-1/2}e^{-|x-y|/\sqrt{\alpha}} \leq C|y|^{-1/2}e^{-|y|/\sqrt{\alpha}}, \]
    then,
    \[ |E(x-y)| \leq C'\,|y|^{-1/2}e^{-|y|/\sqrt{\alpha}}. \]
    Therefore
    \[ |v_\omega(y)| \leq C_1\, |y|^{-1/2}e^{-|y|/\sqrt{\alpha}}\, \|\phi\|_{1/2,\partial B_1}. \]
    
    Next,
    \[ \partial_{y_i} v_\omega(y) = \partial_{y_i}\int_{\partial B_1} E(y-x) p(x)\ d\sigma(x) = \int_{\partial B_1} \partial_{y_i} E(y-x) p(x)\ d\sigma(x), \]
    and
    \[ \partial_{y_i} E(x-y) = \frac{1}{2\pi} \partial_{y_i} K_0(\alpha^{-1/2}|x-y|) = \frac{-1}{2\pi}\alpha^{-1/2}\,|y-x|^{-1}K_1(\alpha^{-1/2}|y-x|)\,y_i. \]
    Thus
    \[ |\nabla v_\omega(y)| = \frac{1}{2\pi}\alpha^{-1/2}\,|y|\,\left|\int_{\partial B_1 }|y-x|^{-1}K_1(\alpha^{-1/2}|y-x|)\,p(x)\ d\sigma(x)\right|, \]
    in the same way that before, for $|y|$ big enough, \cite{Oldham2009},
    \[ |\nabla v_\omega(y)| \leq C\, |y|^{-1/2}e^{-|y|/\sqrt{\alpha}}\, \|\phi\|_{1/2,\partial B_1}. \]
\end{proof}
