# Supplementary material for: Adjoint Method in PDE-based Image Compression
Source: arXiv:2302.02665 source file (2024-10-10)
Supplement: Supplementary file 5 [file appendix03.tex]

\subsection{Some Estimates for the Various Elliptic Problems in the Previous Sections}
\label{appendix:estimates}

In this appendix, we give the estimates of the solution of the problem below with the norms defined in Appendix \ref{appendix:norms}. \\

\begin{proposition} Let $\psi\in H^{1/2}(\partial B_\varepsilon)$ and $\phi\in H^{1/2}(\partial B_R)$. Let $v_\varepsilon$ be the solution of the problem below : 
    \[ \left \{ \begin{array}{cl}
        -\alpha\Delta v_\varepsilon + v_\varepsilon = 0, & \text{in}\ B_R\setminus B_\varepsilon, \\
        v_\varepsilon = \psi, & \text{on}\ \partial B_\varepsilon, \\
        v_\varepsilon = \phi, & \text{on}\ \partial B_R.
    \end{array} \right .\]
    Then, for $\varepsilon$ small enough,
    \begin{align*}
        \|v_\varepsilon\|_{0,B_R\setminus B_\varepsilon} & \leq C_1\,\big(\|\phi\|_{1/2,\partial B_R} + e^{-R/(2\varepsilon\sqrt{\alpha})}\,\|\psi(\varepsilon\,\cdot)\|_{1/2,\partial B_1}\big), \\
        |v_\varepsilon|_{1,B_R\setminus B_\varepsilon} & \leq C_2\,\big(\|\phi\|_{1/2,\partial B_R} + e^{-R/(2\varepsilon\sqrt{\alpha})}\,\|\psi(\varepsilon\,\cdot)\|_{1/2,\partial B_1}\big), \\
        \|v_\varepsilon\|_{0,B_R\setminus B_{R/2}} & \leq C_3\,\big(\|\phi\|_{1/2,\partial B_R} + e^{-R/(2\varepsilon\sqrt{\alpha})}\,\|\psi(\varepsilon\,\cdot)\|_{1/2,\partial B_1}\big), \\
        |v_\varepsilon|_{1,B_R\setminus B_{R/2}} & \leq C_4\,\big(\|\phi\|_{1/2,\partial B_R} + e^{-R/(2\varepsilon\sqrt{\alpha})}\,\|\psi(\varepsilon\,\cdot)\|_{1/2,\partial B_1}\big).
    \end{align*}
    \label{prop:v-epsilon-estimates}
\end{proposition}

The proposition above can be derived easily from the results bellow : \\

\begin{lemma} Let $\phi\in H^{1/2}(\partial B_R)$. Let $v_\varepsilon$ be the solution of the following problem :
    \[ \left \{ \begin{array}{cl}
        -\alpha\Delta v_\varepsilon + v_\varepsilon = 0, & \text{in}\ B_R\setminus B_\varepsilon, \\
        v_\varepsilon = 0, & \text{on}\ \partial B_\varepsilon, \\
        v_\varepsilon = \phi, & \text{on}\ \partial B_R.
    \end{array} \right .\]
    Then, it exists $0<\varepsilon_0<R$ and $C>0$ such that, for all $0<\varepsilon<\varepsilon_0$, we have
    \[ \|v_\varepsilon\|_{1,B_R\setminus B_\varepsilon} \leq C\|\phi\|_{1/2,\partial B_R}. \]
    \label{prop:estimate-1}
\end{lemma}
\begin{proof}
    Let $R/2<\varepsilon_0<R$, them it is readily checked that : 
    \[ \|v_{\varepsilon_0}\|_{1,\alpha,B_R\setminus B_{\varepsilon_0}} \leq C \|v\|_{1,B_R\setminus B_{R/2}}. \]
    Next, we take $\varepsilon < \varepsilon_0$. Then, $D_{\varepsilon_0}\subset D_\varepsilon$ and we denote by $\widetilde{v}_{\varepsilon_0}$ the extension by $0$ of $v_{\varepsilon_0}$ to $D_\varepsilon$. As $v_\varepsilon$ is solution of the problem, it follows :
    \[ \|v_\varepsilon\|_{1,B_R\setminus B_\varepsilon} \leq C\|v_\varepsilon\|_{1,\alpha,B_R\setminus B_\varepsilon}. \]
\end{proof}

\begin{lemma} Let $\psi\in H^{1/2}(\partial B_\varepsilon)$. Let $v_\varepsilon$ be the solution of the following problem :
    \[ \left \{ \begin{array}{cl}
        -\alpha\Delta v_\varepsilon + v_\varepsilon = 0, & \text{in}\ B_R\setminus B_\varepsilon, \\
        v_\varepsilon = \psi, & \text{on}\ \partial B_\varepsilon, \\
        v_\varepsilon = 0, & \text{on}\ \partial B_R.
    \end{array} \right .\]
    Then, for $\varepsilon$ small enough,
    \begin{align*}
        \|v_\varepsilon\|_{0,B_R\setminus B_\varepsilon} & \leq C_1\,e^{-R/(2\varepsilon\sqrt{\alpha})}\,\|\psi(\varepsilon\,\cdot)\|_{1/2,\partial B_1}, \\
        |v_\varepsilon|_{1,B_R\setminus B_\varepsilon} & \leq C_2\,e^{-R/(2\varepsilon\sqrt{\alpha})}\,\|\psi(\varepsilon\,\cdot)\|_{1/2,\partial B_1}, \\
        \|v_\varepsilon\|_{0,B_R\setminus B_{R/2}} & \leq C_3\,e^{-R/(2\varepsilon\sqrt{\alpha})}\,\|\psi(\varepsilon\,\cdot)\|_{1/2,\partial B_1} \\
        |v_\varepsilon|_{1,B_R\setminus B_{R/2}} & \leq C_4\,e^{-R/(2\varepsilon\sqrt{\alpha})}\,\|\psi(\varepsilon\,\cdot)\|_{1/2,\partial B_1}.
    \end{align*}
\end{lemma}
\begin{proof}
    We consider the following \textit{exterior} problem : 
    \[ \left \{ \begin{array}{cl}
        -\alpha\Delta v_{\omega_\varepsilon} + v_{\omega_\varepsilon} = 0, & \text{in}\ \R^2\setminus B_1, \\
        v_{\omega_\varepsilon} = \psi(\varepsilon\,\cdot), & \text{on}\ \partial B_1, \\
        v_{\omega_\varepsilon} = 0, & \text{at}\ \infty.
    \end{array} \right .\]
    Therefore,
    \[ v_\varepsilon = v_{\omega_\varepsilon}(\cdot/\varepsilon)|_{B_R\setminus B_\varepsilon} - w_\varepsilon, \]
    where $w_\varepsilon$ is solution of
    \[ \left \{ \begin{array}{cl}
        -\alpha\Delta w_\varepsilon + w_\varepsilon = 0, & \text{in}\ B_R\setminus B_\varepsilon, \\
        w_\varepsilon = 0, & \text{on}\ \partial B_\varepsilon, \\
        w_\varepsilon = v_{\omega_\varepsilon}(\cdot/\varepsilon), & \text{on}\ \partial B_R.
    \end{array} \right .\]
    Using Proposition \ref{prop:estimate-1} and Proposition \ref{prop:exterior-pb-estimates}, for $\varepsilon$ small enough, we have
    \begin{align*}
        \|w_\varepsilon\|_{1,B_R\setminus B_\varepsilon} & \leq C\, e^{-R/(2\varepsilon\sqrt{\alpha})}\,\|\psi(\varepsilon\,\cdot)\|_{1/2,\partial B_1}.
    \end{align*}
    It follows from scaling argument, 
    \begin{align*}
        \|v_\varepsilon\|_{0,B_R\setminus B_\varepsilon} & \leq \|v_{\omega_\varepsilon}(\cdot/\varepsilon)\|_{0,B_R\setminus B_\varepsilon} + \|w_\varepsilon\|_{0,B_R\setminus B_\varepsilon} \\ 
        & \leq C\,e^{-R/(2\varepsilon\sqrt{\alpha})}\,\|\psi(\varepsilon\,\cdot)\|_{1/2,\partial B_1}.
    \end{align*}
    The other estimations are obtained similarly.
\end{proof}
