# Supplementary material for: Adjoint Method in PDE-based Image Compression
Source: arXiv:2302.02665 source file (2024-10-10)
Supplement: Supplementary file 6 [file appendix04.tex]

\section{Étude du Problème Extérieur}

\subsection{Trou normalisé}

Pour $\beta\in\R$,

\[ \left \{ \begin{array}{cc}
    -\alpha\Delta v_\omega + v_\omega = 0, & \text{dans}\ \R^2\setminus B(0,1), \\
    v_\omega = \beta, & \text{sur}\ \partial B(0,1), \\
    v_\omega = 0, & \text{à}\ \infty.
\end{array}
\right .\]

\begin{proposition}
    \[ v_\omega(y) = \beta \Big(K_0\big(\alpha^{-1/2}\big)\Big)^{-1} K_0\left(\frac{1}{\sqrt{\alpha}}|y|\right). \]
\end{proposition}
\begin{proof}
    Comme le trou est une boule, la solution est radiale.
    
    \[ E(y) := \frac{1}{2\pi} K_0\left(\frac{1}{\sqrt{\alpha}}|y|\right). \]
    
    \[ v_\omega(y) = \beta\frac{1}{E(1)}E(y) = \beta \Big(K_0\big(\alpha^{-1/2}\big)\Big)^{-1} K_0\left(\frac{1}{\sqrt{\alpha}}|y|\right). \]
\end{proof}

\begin{proposition}
    \[ \|v_\omega\|_{L^2(B_{R/\varepsilon}\setminus B_1)} \leq \pi^{1/2} R\varepsilon^{-1} |\beta|,  \]
    \[ |v_\omega|_{H^1(B_{R/\varepsilon}\setminus B_1)} \leq  \pi^{1/2} R\varepsilon^{-1}\alpha^{-1/2} |\beta|, \]
    \[ \|v_\omega\|_{H^1(B_{R/\varepsilon}\setminus B_1)} \leq  \pi^{1/2} R\varepsilon^{-1} (1+\alpha^{-1/2}) |\beta|. \]
\end{proposition}
\begin{proof}
    Soit $y$ dans $\R^2\setminus B(x_0,1)$. Puisque $K_0$ est décroissante sur $\R$,
    
    \[ |v_\omega(y)|\leq |\beta| \Big(K_0\big(\alpha^{-1/2}\big)\Big)^{-1} K_0\left(\frac{1}{\sqrt{\alpha}}\right) = |\beta|. \]
    
    D'où
    
    \[ \|v_\omega\|_{L^2(B_{R/\varepsilon}\setminus B_1)}^2 = \int_{B_{R/\varepsilon}\setminus B_1} v_\omega^2\ dx \leq \pi (R/\varepsilon-1)^2 |\beta|^2 \leq \pi R^2\varepsilon^{-2} |\beta|^2, \]
    
    et
    
    \[ |v_\omega|_{H^1(B_{R/\varepsilon}\setminus B_1)}^2 = \int_{B_{R/\varepsilon}\setminus B_1} |\nabla v_\omega|^2\ dx = \frac{1}{\alpha} \int_{\partial B_{R/\varepsilon}}v_\omega \partial_n v_\omega \ d\sigma + \frac{1}{\alpha} \int_{\partial B_1}v_\omega \partial_n v_\omega \ d\sigma + \frac{1}{\alpha}\int_{B_{R/\varepsilon}\setminus B_1} v_\omega^2\ dx \]
    
    Puisque $v_\omega$ est radiale, on peut facilement calculer la dérivée normale à une boule,
    
    \[ |v_\omega|_{H^1(B_{R/\varepsilon}\setminus B_1)}^2 = -2\pi R \varepsilon^{-1} \alpha^{-3/2} \beta^2 \Big(K_0\big(\alpha^{-1/2}\big)\Big)^{-2}K_0\big(\alpha^{-1/2}R/\varepsilon\big)K_1\big(\alpha^{-1/2}R/\varepsilon\big) \]\[ -2\pi \alpha^{-3/2} \beta^2 \Big(K_0\big(\alpha^{-1/2}\big)\Big)^{-2}K_0\big(\alpha^{-1/2}\big)K_1\big(\alpha^{-1/2}\big) + \frac{1}{\alpha}\int_{B_{R/\varepsilon}\setminus B_1} v_\omega^2\ dx \]
    
    Comme $K_0$ et $K_1$ sont positifs,
    
    \[ |v_\omega|_{H^1(B_{R/\varepsilon}\setminus B_1)}^2 \leq \frac{1}{\alpha}\int_{B_{R/\varepsilon}\setminus B_1} v_\omega^2\ dx \leq \pi R^2\varepsilon^{-2}  \alpha^{-1}|\beta|^2. \]
\end{proof}

\subsection{Trou $\epsilon$}

\[ \left \{ \begin{array}{cc}
    -\alpha\Delta v_{\omega_\varepsilon} + v_{\omega_\varepsilon} = 0, & \text{dans}\ \R^2\setminus B(0,\varepsilon), \\
    v_{\omega_\varepsilon} = \beta, & \text{sur}\ \partial B(0,\varepsilon), \\
    v_{\omega_\varepsilon} = 0, & \text{à}\ \infty.
\end{array}
\right .\]

\begin{proposition}
    \[ v_{\omega_\varepsilon}(y) = v_\omega(y/\varepsilon), \]
    
    et pour $\varepsilon<1$
    
    \[ \|v_{\omega_\varepsilon}\|_{L^2(B_R\setminus B_\varepsilon)} \leq \pi^{1/2} R\varepsilon^{-1/2} |\beta|,  \]
    \[ |v_{\omega_\varepsilon}|_{H^1(B_R\setminus B_\varepsilon)} \leq \pi^{1/2} R\varepsilon^{-3/2} \alpha^{-1/2} |\beta|, \]
    \[ \|v_{\omega_\varepsilon}\|_{H^1(B_R\setminus B_\varepsilon)} \leq 2\pi^{1/2} R\varepsilon^{-3/2} \alpha^{-1/2} |\beta|. \]
\end{proposition}
\begin{proof}
    \[ \|v_{\omega_\varepsilon}\|_{L^2(B_R\setminus B_\varepsilon)}^2 = \int_{B_R\setminus B_\varepsilon}v_{\omega_\varepsilon}(x)^2\ dx = \int_{B_R\setminus B_\varepsilon}v_\omega(x/\varepsilon)^2\ dx = \varepsilon\int_{B_{R/\varepsilon}\setminus B_1}v_\omega(y)^2\ dy, \]
    
    Aussi
    
    \[  |v_{\omega_\varepsilon}|_{H^1(B_R\setminus B_\varepsilon)}^2 = \int_{B_R\setminus B_\varepsilon} |\nabla v_{\omega_\varepsilon}(x)|^2\ dx = \int_{B_R\setminus B_\varepsilon} |\nabla v_\omega(x/\varepsilon)|^2\ dx = \varepsilon^{-1}\int_{B_{R/\varepsilon}\setminus B_1} |\nabla v_\omega(y)|^2\ dy.  \]
\end{proof}

\subsection{Extérieur tronqué}

On propose d'étudier \[ h_\omega := (v_{\omega_\varepsilon} - v_{\omega_\varepsilon}|_{\partial B_R})|_{B_R\setminus B_\varepsilon}. \]

\begin{proposition}

    \[ \left \{ \begin{array}{cc}
        -\alpha\Delta h_\omega + h_\omega = 0, & \text{dans}\ B_R\setminus B(0,\varepsilon), \\
        h_\omega = \beta \left(1- \Big(K_0\big(\alpha^{-1/2}\big)\Big)^{-1} K_0\left(\frac{R}{\epsilon\sqrt{\alpha}}\right)\right), & \text{sur}\ \partial B(0,\varepsilon), \\
        h_\omega = 0, & \text{sur}\ \partial B(0,R).
    \end{array}
    \right .\]

    \[ h_\omega = \beta \Big(K_0\big(\alpha^{-1/2}\big)\Big)^{-1}\left( K_0\left(\frac{1}{\varepsilon\sqrt{\alpha}}|y|\right) - K_0\left(\frac{R}{\varepsilon\sqrt{\alpha}}\right)\right). \]
\end{proposition}
\begin{proof}
    \[ h_\omega = (v_{\omega_\varepsilon} - v_{\omega_\varepsilon}|_{\partial B_R})|_{B_R\setminus B_\varepsilon}... \]
\end{proof}
\begin{note}
    $K_0$ décroissante et $K_0>0$ donc $h_\omega<0$?
\end{note}

\subsection{Approximation de la variation de la solution}

\[ \mathcal{E} = h_\varepsilon - h_\omega =  \]

\[ \left \{ \begin{array}{cc}
    -\alpha\Delta \mathcal{E} + \mathcal{E} = 0, & \text{dans}\ B_R \setminus B(0,\varepsilon), \\
    \mathcal{E} = v_0^{g,\phi} - v_D(x_0) \left(1- \Big(K_0\big(\alpha^{-1/2}\big)\Big)^{-1} K_0\left(\frac{R}{\epsilon\sqrt{\alpha}}\right)\right), & \text{sur}\ \partial B(0,\varepsilon), \\
    \mathcal{E} = 0, & \text{sur}\ \partial B(0,R).
\end{array}
\right .\]

Formulation variationnelle pour $\varphi\in V_R$

\[ -\alpha\int_{B_R\setminus B_\varepsilon}\Delta\mathcal{E}\varphi\ dx + \int_{B_R\setminus B_\varepsilon}\mathcal{E}\varphi\ dx = 0 \]

\[ \alpha\int_{B_R\setminus B_\varepsilon}\nabla\mathcal{E}\cdot\nabla\varphi\ dx - \alpha\int_{\partial B_R}\partial_n\mathcal{E}\varphi\ d\sigma - \alpha\int_{\partial B_\varepsilon}\partial_n\mathcal{E}\varphi\ d\sigma + \int_{B_R\setminus B_\varepsilon}\mathcal{E}\varphi\ dx = 0 \]

\[ \alpha\int_{B_R\setminus B_\varepsilon}\nabla\mathcal{E}\cdot\nabla\varphi\ dx - \alpha\int_{\partial B_\varepsilon}\partial_n\mathcal{E}\varphi\ d\sigma + \int_{B_R\setminus B_\varepsilon}\mathcal{E}\varphi\ dx = 0 \]

On prend comme fonction test $\mathcal{E}$

\[ \alpha\int_{B_R\setminus B_\varepsilon}|\nabla\mathcal{E}|^2\ dx - \alpha\int_{\partial B_\varepsilon}\mathcal{E}\partial_n\mathcal{E}\ d\sigma + \int_{B_R\setminus B_\varepsilon}\mathcal{E}^2\ dx = 0 \]

\[ \alpha\int_{B_R\setminus B_\varepsilon}|\nabla(h_\varepsilon - h_\omega)|^2\ dx + \int_{B_R\setminus B_\varepsilon}(h_\varepsilon - h_\omega)^2\ dx = \alpha\int_{\partial B_\varepsilon}(h_\varepsilon - h_\omega)\partial_n(h_\varepsilon - h_\omega)\ d\sigma \]

Avec un changement de variable $y=\varepsilon x$ (ou un truc du genre)

\[ \alpha\varepsilon^{-1}\int_{B_R\setminus B_1}|\nabla(h_\varepsilon - h_\omega)|^2\ dy + \varepsilon^{-1}\int_{B_R\setminus B_1}(h_\varepsilon - h_\omega)^2\ dy = \alpha\int_{\partial B_\varepsilon}(h_\varepsilon - h_\omega)\partial_n(h_\varepsilon - h_\omega)\ d\sigma \]

\[ \alpha\varepsilon^{-1}\int_{B_R\setminus B_1}|\nabla(h_\varepsilon - h_\omega)|^2\ dy + \varepsilon^{-1}\int_{B_R\setminus B_1}(h_\varepsilon - h_\omega)^2\ dy = \alpha\int_{\partial B_\varepsilon}(h_\varepsilon - h_\omega)\partial_n(h_\varepsilon - h_\omega)\ d\sigma \]

\[ \varepsilon^{-1}\|h_\varepsilon - h_\omega\|_{V_R,\alpha}^2 = \alpha\int_{\partial B_\varepsilon}(h_\varepsilon - h_\omega)\partial_n(h_\varepsilon - h_\omega)\ d\sigma \]

\[ \varepsilon^{-1}\|h_\varepsilon - h_\omega\|_{V_R,\alpha}^2 = \alpha\int_{\partial B_\varepsilon}(h_\varepsilon - h_\omega)\partial_n(h_\varepsilon - h_\omega)\ d\sigma \]

\[ \varepsilon^{-1}\|h_\varepsilon - h_\omega\|_{V_R,\alpha}^2 = \alpha v_D(x_0) \left(1- \Big(K_0\big(\alpha^{-1/2}\big)\Big)^{-1} K_0\left(\frac{R}{\epsilon\sqrt{\alpha}} \right)\right)\left(\int_{\partial B_\varepsilon}v_0^{g,\phi}\partial_n h_\omega\ d\sigma- \int_{\partial B_\varepsilon} v_0^{g,\phi}\partial_n h_\varepsilon\ d\sigma\right) \]

avec un changement de variable approprié

\[ \varepsilon^{-1}\|h_\varepsilon - h_\omega\|_{V_R,\alpha}^2 = \alpha v_D(x_0) \left(1- \Big(K_0\big(\alpha^{-1/2}\big)\Big)^{-1} K_0\left(\frac{R}{\epsilon\sqrt{\alpha}} \right)\right)\varepsilon^{-1}\left(\int_{\partial B_1}v_0^{g,\phi}\partial_n h_\omega\ d\sigma- \int_{\partial B_1} v_0^{g,\phi}\partial_n h_1\ d\sigma\right) \]

\[ \varepsilon^{-1}\|h_\varepsilon - h_\omega\|_{V_R,\alpha}^2 \leq \alpha v_D(x_0) \left(1- \Big(K_0\big(\alpha^{-1/2}\big)\Big)^{-1} K_0\left(\frac{R}{\epsilon\sqrt{\alpha}} \right)\right)\varepsilon^{-1}C\]

Pour $\varepsilon$ suffisamment petit, on a 

\[ \|h_\varepsilon - h_\omega\|_{V_R,\alpha}^2 \leq \alpha v_D(x_0) \left(1- C_2 \sqrt{\frac{\pi}{2}}\frac{e^{-1/\varepsilon}}{\sqrt{1/\varepsilon}} \right)C_1 + O\left(\frac{e^{-1/\varepsilon}}{\sqrt{1/\varepsilon}}\right)\]

\subsection{Approximation de la variation de la solution - Tentative n°2}

Pour $\varphi \in H^1(D\setminus B_R)$,

\[ \alpha\int_{B_R\setminus B_\varepsilon} \nabla(h_\varepsilon - h_\omega)\cdot\nabla\varphi\ dx - \int_{\partial B_R\cup\partial B_\varepsilon} \partial_n(h_\varepsilon - h_\omega)\varphi\ d\sigma + \int_{D_\varepsilon} (h_\varepsilon - h_\omega)\varphi\ dx \]

\subsection{Approximation de la variation de la solution - Tentative n°3}

J'écrit $v_0$ et $v_\varepsilon$ à la place de $v_0^{g,\phi}$ et $v_\varepsilon^{g,\phi}$

\[ -\alpha\int_{D_\varepsilon} \Delta(v_0(y) - v_\varepsilon(y) - v_\omega(y/\varepsilon))\varphi\ dy + \int_{D_\varepsilon} (v_0(y) - v_\varepsilon(y) - v_\omega(y/\varepsilon))\varphi\ dy \]

\[ = \alpha\int_{D_\varepsilon} \nabla(v_0(y) - v_\varepsilon(y) - v_\omega(y/\varepsilon))\cdot\nabla\varphi\ dy -\alpha\int_{\partial D_\varepsilon} \partial_n(v_0(y) - v_\varepsilon(y) - v_\omega(y/\varepsilon))\varphi\ d\sigma +
\int_{D_\varepsilon} (v_0(y) - v_\varepsilon(y) - v_\omega(y/\varepsilon))\varphi\ dy \]

\[ = \alpha\int_{D_\varepsilon} \nabla(v_0(y) - v_\varepsilon(y) - v_\omega(y/\varepsilon))\cdot\nabla\varphi\ dy +
\int_{D_\varepsilon} (v_0(y) - v_\varepsilon(y) - v_\omega(y/\varepsilon))\varphi\ dy - \alpha\int_{\partial D_\varepsilon} \partial_n(v_0(y) - v_\varepsilon(y) - v_\omega(y/\varepsilon))\varphi\ d\sigma \]

\[ \left \{ \begin{array}{cc}
    -\alpha\Delta\big(v_0(y) - v_\varepsilon(y) - v_\omega(y/\varepsilon)\big) + \big(v_0(y) - v_\varepsilon(y) - v_\omega(y/\varepsilon)\big) = 0, & \text{dans}\ B_R\setminus B_\varepsilon, \\
    \big(v_0(y) - v_\varepsilon(y) - v_\omega(y/\varepsilon)\big) = v_0(y) - v_0(x_0), & \text{sur}\ \partial B_\varepsilon, \\
    \big(v_0(y) - v_\varepsilon(y) - v_\omega(y/\varepsilon)\big) = - v_\omega(y/\varepsilon), & \text{sur}\ \partial B_R.
\end{array} \right .\]

\section{Calculs}

On pose $h_\varepsilon^{g,\phi} := v_0^{g,\phi} - v_\varepsilon^{g,\phi}$. Alors 

\[ \left \{ \begin{array}{cc}
    -\alpha\Delta h_\varepsilon^{g,\phi} + h_\varepsilon^{g,\phi} = 0, & \text{dans}\ B_R\setminus B_\varepsilon, \\
    h_\varepsilon^{g,\phi} = v_0^{g,\phi}, & \text{sur}\ \partial B_\varepsilon, \\
    h_\varepsilon^{g,\phi} = 0, & \text{sur}\ \partial B_R.
\end{array} \right .\]

Principe du max : 

\[ \max |h_\varepsilon| = \max_{\partial B_\varepsilon} |v_0| \]

\begin{lemma}[Solution fondamentale]
    \[ E(y) := \frac{1}{2\pi} K_0\left(\frac{1}{\sqrt{\alpha}}|y|\right) \]
    
    Alors 
    
    \[ -\alpha\Delta E + E = 0. \]
\end{lemma}

On peut prendre $x_0=0$ pour être plus simple mais ça change rien. \\

\begin{lemma}[Problème extérieur]
    \[ \left \{ \begin{array}{cc}
        -\alpha\Delta v_{\omega_\varepsilon} + v_{\omega_\varepsilon} = 0, & \text{dans}\ \R^2\setminus B(0,\varepsilon), \\
        v_{\omega_\varepsilon} = v_D(x_0), & \text{sur}\ \partial B(0,\varepsilon), \\
        v_{\omega_\varepsilon} = 0, & \text{à}\ \infty.
    \end{array}
    \right .\]
    
    Alors on a pour $|y|$ suffisamment grand,
    
    \[ v_{\omega_\varepsilon}(y) = \frac{v_D(x_0)}{E(\varepsilon)}E(y). \]
\end{lemma}
\begin{proof}
    Comme le trou est une boule, la solution est radiale.
\end{proof}

On pose $z_\varepsilon^{g,\phi} := h_\varepsilon^{g,\phi} - \big(v_{\omega_\varepsilon} - v_{\omega_\varepsilon}|_{\partial B_R}\big)|_{B_R\setminus B_\varepsilon}$. Alors, $z_\varepsilon^{g,\phi}$ est solution de

\[ \left \{ \begin{array}{cc}
    -\alpha\Delta z_\varepsilon^{g,\phi} + z_\varepsilon^{g,\phi} = 0, & \text{dans}\ B_R\setminus B_\varepsilon, \\
    z_\varepsilon^{g,\phi} = v_0^{g,\phi} - v_D(x_0) + v_{\omega_\varepsilon}|_{\partial B_\varepsilon}, & \text{sur}\ \partial B_\varepsilon, \\
    z_\varepsilon^{g,\phi} = 0, & \text{sur}\ \partial B_R.
\end{array} \right .\]

Sur $\partial B_\varepsilon,$

\[ z_\varepsilon^{g,\phi} = v_0^{g,\phi}|_{B_\varepsilon} - v_D(x_0) + v_{\omega_\varepsilon}|_{\partial B_\varepsilon} = v_0^{g,\phi}|_{B_\varepsilon} - v_D(x_0)\left(1-\frac{E(R)}{E(\varepsilon)}\right) \]

On remarque que \[ z_\varepsilon^{g,\phi}(y/\varepsilon) = z_1^{g,\phi}(y). \]
