# Supplementary material for: Adjoint Method in PDE-based Image Compression
Source: arXiv:2302.02665 source file (2024-10-10)
Supplement: Supplementary file 7 [file appendix04b.tex]

\section{Preliminaries}
\subsection{Recall on the Sobolev Norms}
\label{appendix:norms}

We recall the definition of the norms and some of their properties used in the proofs. Let $\mathcal{O}$ be an open subset of $\R^2$. For $v$ in $H^1(\mathcal{O})$, we recall the following Sobolev norms :
% \begin{align*}
%     & \|v\|_{0,\mathcal{O}} := \left(\int_\mathcal{O} v^2\ dx \right)^{1/2}, \\
%     %
%     & |v|_{1,\mathcal{O}} := \left(\int_\mathcal{O}|\nabla v|^2\ dx\right)^{1/2}, \\
%     %
%     & \|v\|_{1,\mathcal{O}} := \left(\int_\mathcal{O} v^2\ dx + \int_\mathcal{O}|\nabla v|^2\ dx\right)^{1/2}, \\
%     %
%     & \|v\|_{1,\alpha,\mathcal{O}} := \left(\int_\mathcal{O} v^2\ dx + \alpha\int_\mathcal{O}|\nabla v|^2\ dx\right)^{1/2}.
% \end{align*}
\[ \begin{array}{ll}
    \|v\|_{0,\mathcal{O}} := \left(\int_\mathcal{O} v^2\ dx \right)^{1/2}, & |v|_{1,\mathcal{O}} := \left(\int_\mathcal{O}|\nabla v|^2\ dx\right)^{1/2}, \\
    \|v\|_{1,\mathcal{O}} := \left(\int_\mathcal{O} v^2\ dx + \int_\mathcal{O}|\nabla v|^2\ dx\right)^{1/2}, & \|v\|_{1,\alpha,\mathcal{O}} := \left(\int_\mathcal{O} v^2\ dx + \alpha\int_\mathcal{O}|\nabla v|^2\ dx\right)^{1/2}.
\end{array} \]

Now we set $\mathcal{O}_\varepsilon := \{ x/\varepsilon\ |\ x\in\mathcal{O} \}$. Straightforward computations give : \\

\begin{proposition}
    % \[ |u|_{1,\mathcal{O}} = |u(\varepsilon\,\cdot\,)|_{1,\mathcal{O}/\varepsilon}, \]
    % \[ \|u\|_{0,\mathcal{O}} = \varepsilon^{-1}\|u(\varepsilon\,\cdot\,)\|_{0,\mathcal{O}/\varepsilon}. \]
    \begin{align*}
        & \|u(\cdot/\varepsilon)\|_{0,\mathcal{O}} = \varepsilon\|u\|_{0,\mathcal{O}_\varepsilon}, \\
        & |u(\cdot/\varepsilon)|_{1,\mathcal{O}} = |u|_{1,\mathcal{O}_\varepsilon}.
    \end{align*}
\end{proposition}
% \begin{proof}
%     For $x$ in $\mathcal{O}\subset \R^2$, we set $y:=x/\varepsilon$. \\

%     \textbullet ~ \textbf{Show (1) :} \\
%     \[ |u|^2_{1,\mathcal{O}} = \int_\mathcal{O}|\nabla u|^2\ dx = \varepsilon^{-2} \int_{\mathcal{O}_\varepsilon} |\nabla(u(\varepsilon\,y))|^2\ dy = \varepsilon^{-2} \int_{\mathcal{O}_\varepsilon} \varepsilon^2|\nabla u(\varepsilon\,y)|^2\ dy = |u(\varepsilon\,\cdot\,)|^2_{1,\mathcal{O}_\varepsilon}. \]
    
%     \textbullet ~ \textbf{Show (2) :} \\
%     \[ \|u\|^2_{0,\mathcal{O}} = \int_\mathcal{O}|u|^2\ dx = \varepsilon^{-2} \int_{\mathcal{O}_\varepsilon} |u(\varepsilon\,y)|^2\ dy = \varepsilon^{-2}\|u(\varepsilon\,\cdot\,)\|^2_{0,\mathcal{O}_\varepsilon}. \]
% \end{proof}

On the boundary of a ball of radius $r>0$, namely $\partial B_r$, we define for $\phi$ in $H^{1/2}(\partial B_r)$, 
\[ \|\phi\|_{1/2,\partial B_r} := \inf_{u=\phi\ \text{on}\ \Gamma} \|u\|_{1,B_r\setminus B_{r/2}}, \]
and for $\psi$ in $H^{-1/2}(\partial B_r)$, we define the dual norm,
\[ \|\psi\|_{-1/2,\partial B_r} := \sup_{v\in H^{1/2}(\partial B_r),\,\|v\|_{1/2,\partial B_r}=1} \int_{\partial B_r} \psi\, v\ d\sigma. \]
Then, it is standard that \\

\begin{proposition} \label{prop:norm-minus-1-2}
    Let $\psi\in H^1(B_R\setminus B_{R/2})$, with $-\alpha\Delta\psi + \psi = 0$ in $B_R\setminus B_{R/2}$, there exists $C>0$, such that
    \[ \|\nabla\psi\cdot n\|_{-1/2,\partial B_R} \leq C\,\|\psi\|_{1,B_R\setminus B_{R/2}}. \]
\end{proposition}
