# Supplementary material for: Adjoint Method in PDE-based Image Compression
Source: arXiv:2302.02665 source file (2024-10-10)
Supplement: Supplementary file 8 [file appendix05.tex]

\newpage

% \begin{lemma}[Problème extérieur]
%     \[ \left \{ \begin{array}{cc}
%         -\alpha\Delta v_\omega + v_\omega = 0, & \text{dans}\ \R^2\setminus B(0,1), \\
%         v_\omega = v_D(x_0), & \text{sur}\ \partial B(0,1), \\
%         v_\omega = 0, & \text{à}\ \infty.
%     \end{array}
%     \right .\]
    
%     Alors on a pour $|y|$ suffisamment grand,
    
%     \[ v_\omega(y) = \frac{1}{2\pi}A\big(v_D(x_0)\big) K_0\left(\frac{1}{\sqrt{\alpha}}|y|\right) + O\left(\frac{e^{-y}}{\sqrt{y}}\right). \]
% \end{lemma}
% \begin{proof}
%     Pour tout $y\in\R^2\setminus B_1$, on a
%     \[ v_\omega(y) = \int_{\partial B_1}E(y-x) p_\omega(x)\ d\sigma(x) \]
%     avec $p_\omega$ solution de 
%     \[  \int_{\partial B_1}E(y-x) p_\omega(x)\ d\sigma(x) = u_D(x_0),\ \forall y\in \partial B_1. \]
    
%     Pour $|y|$ suffisament grand, on a
    
%     \[ E(y-x) = E(y) + O\left(\sqrt{\frac{\pi}{2}} \frac{e^{-y}}{\sqrt{y}}\right). \]
    
%     Un développement asymptotique à l'infini nous donne 
    
%     \[ v_\omega(y) = E(y)\int_{\partial B_1} p_\omega(x)\ d\sigma(x) + O\left(\frac{e^{-y}}{\sqrt{y}}\right) \]
%     \[ = \frac{1}{2\pi} K_0\left(\frac{1}{\sqrt{\alpha}}|y|\right)\int_{\partial B_1} p_\omega(x)\ d\sigma(x) + O\left(\frac{e^{-y}}{\sqrt{y}}\right) \]
    
%     \[ = \frac{1}{2\pi}A\big(v_D(x_0)\big) K_0\left(\frac{1}{\sqrt{\alpha}}|y|\right) + O\left(\frac{e^{-y}}{\sqrt{y}}\right) \]
% \end{proof}
\begin{note}
    On a en quelques sortes (pas exactement à cause de $\partial B_\varepsilon$) \[ h_\varepsilon\to_{R\to+\infty} v_{\omega_\varepsilon}, \]
    lorsque $\phi = v_D|_{\partial B_R}$.
\end{note} ~ \\

\begin{lemma}
    \[ v_\omega(y) = v_D(x_0)\frac{\sqrt{2}\pi^{3/2}}{K_0\big(\alpha^{-1/2}\big)}\frac{e^{-|y|}}{\sqrt{|y|}} + O\left(\frac{e^{-|y|}}{\sqrt{|y|}}\right). \]
\end{lemma}
\begin{proof}
    D'après \cite{Oldham2009}, pour $|y|$ grand, on a
    
    \[ E(y) = \sqrt{\frac{\pi}{2}}\frac{e^{-|y|}}{\sqrt{|y|}} + O\left(\frac{e^{-|y|}}{\sqrt{|y|}}\right) \]
\end{proof}

% \begin{lemma}[Problème extérieur]
%     \[ \left \{ \begin{array}{cc}
%         -\alpha\Delta v_{\omega_\varepsilon} + v_{\omega_\varepsilon} = 0, & \text{dans}\ \R^2\setminus B(0,\varepsilon), \\
%         v_{\omega_\varepsilon} = v_D(x_0), & \text{sur}\ \partial B(0,\varepsilon), \\
%         v_{\omega_\varepsilon} = 0, & \text{à}\ \infty.
%     \end{array}
%     \right .\]
    
%     Alors on a pour $|y|$ suffisamment grand,
    
%     \[ v_{\omega_\varepsilon} = v_D(x_0)\frac{\sqrt{2}\pi^{3/2}}{K_0\big(\alpha^{-1/2}\big)}\frac{e^{-\varepsilon|y|}}{\sqrt{\varepsilon|y|}} + O\left(\frac{e^{-\varepsilon|y|}}{\sqrt{\varepsilon|y|}}\right). \]
% \end{lemma}
% \begin{proof}
%     \[ v_{\omega_\varepsilon}(y) = v_\omega(\varepsilon y). \]
% \end{proof}

\begin{lemma}
    \[ v_\varepsilon^{g,\phi} - v_0^{g,\phi} = \varepsilon (Q_\omega - P_\omega) + O\left(\frac{e^{-|y|}}{\sqrt{|y|}}\right), \]
    
    avec
    \[ P_\omega :=  v_D(x_0)\frac{\sqrt{2}\pi^{3/2}}{K_0\big(\alpha^{-1/2}\big)}\frac{e^{-|y|}}{\sqrt{|y|}}, \]
    et
    \[ Q_\omega := P_\omega|_{\partial B_R} =  v_D(x_0)\frac{\sqrt{2}\pi^{3/2}}{K_0\big(\alpha^{-1/2}\big)}\frac{e^{-R}}{\sqrt{R}}. \]
\end{lemma}
\begin{proof}
    \[ v_\varepsilon^{g,\phi} - v_0^{g,\phi} = -h_\varepsilon^{g,\phi} \]
\end{proof}

\newpage

\begin{lemma}
    Pour $0<\varepsilon<R$,
    \[ v_\varepsilon^{g,\phi} - v_0^{g,\phi} = \frac{1}{2\pi}A\big(v_D(x_0)\big)\left( K_0\left(\frac{1}{\sqrt{\alpha}}R\right) -\frac{1}{2}\ln{\alpha} - \ln{2} + \gamma \right)\varepsilon + \frac{1}{2\pi}A\big(v_D(x_0)\big)\varepsilon\ln{|y|} + O(\varepsilon) + O(\varepsilon|y|^2\ln{|y|}), \]
    lorsque $\phi = v_D|_{\partial B_R}$.
\end{lemma}
\begin{proof}
    
    Pour $0<|y|<\varepsilon$,

    \[ v_\varepsilon^{g,\phi} - v_0^{g,\phi} = \varepsilon \left( \frac{1}{2\pi}A\big(v_D(x_0)\big) K_0\left(\frac{1}{\sqrt{\alpha}}R\right) - \frac{1}{2\pi}A\big(v_D(x_0)\big) K_0\left(\frac{1}{\sqrt{\alpha}}|y|\right) \right) + O(\varepsilon), \]
    
    Pour $\varepsilon$ petit, on a 
    
    \[ K_0\left(\frac{1}{\sqrt{\alpha}}|y|\right) = -\ln{|y|} +\frac{1}{2}\ln{\alpha} + \ln{2} - \gamma + O(|y|^2\ln{|y|}). \]

    D'où
    
    \[ v_\varepsilon^{g,\phi} - v_0^{g,\phi} =  \frac{1}{2\pi}A\big(v_D(x_0)\big) K_0\left(\frac{1}{\sqrt{\alpha}}R\right)\varepsilon - \frac{1}{2\pi}A\big(v_D(x_0)\big) K_0\left(\frac{1}{\sqrt{\alpha}}|y|\right)\varepsilon + O(\varepsilon) \]
    \[ = \frac{1}{2\pi}A\big(v_D(x_0)\big)\left( K_0\left(\frac{1}{\sqrt{\alpha}}R\right) -\frac{1}{2}\ln{\alpha} - \ln{2} + \gamma \right)\varepsilon + \frac{1}{2\pi}A\big(v_D(x_0)\big)\varepsilon\ln{|y|} + O(\varepsilon) + O(\varepsilon|y|^2\ln{|y|}). \]
\end{proof}

\begin{lemma}
    \[ \int_{\partial B_R}\partial_n (v_\varepsilon^{g,\phi} - v_0^{g,\phi})\ d\sigma = A\big(v_D(x_0)\big)\frac{\varepsilon}{R} + O(\varepsilon) \]
\end{lemma}
\begin{proof}
    \[ \int_{\partial B_R}\partial_n (v_\varepsilon^{g,\phi} - v_0^{g,\phi})\ d\sigma = \] \[\int_{\partial B_R}\partial_n (\frac{1}{2\pi}A\big(v_D(x_0)\big)\left( K_0\left(\frac{1}{\sqrt{\alpha}}R\right) -\frac{1}{2}\ln{\alpha} - \ln{2} + \gamma \right)\varepsilon + \frac{1}{2\pi}A\big(v_D(x_0)\big)\varepsilon\ln{|y|} + O(\varepsilon) + O(\varepsilon|y|^2\ln{|y|}))\ d\sigma \]
    \[ = \int_{\partial B_R}\partial_n ( \frac{1}{2\pi}A\big(v_D(x_0)\big)\varepsilon\ln{|y|} + O(\varepsilon|y|^2\ln{|y|}))\ d\sigma \]
    \[ = \frac{1}{2\pi}A\big(v_D(x_0)\big)\varepsilon\int_{\partial B_R}\partial_n ( \ln{|y|} )\ d\sigma + O(\varepsilon) \int_{\partial B_R}\partial_n (|y|^2\ln{|y|})\ d\sigma \]
    
    De plus,
    
    \[ \int_{\partial B_R}\partial_n ( \ln{|y|} )\ d\sigma = 2\pi \frac{1}{R} \]
    et 
    \[ \int_{\partial B_R}\partial_n (|y|^2\ln{|y|})\ d\sigma = 2\pi (2R\ln{R} + R) \]
\end{proof}

\begin{note}
    \cite{Peter2019} On propose en $1D$ de calculer explicitement $v_0\,w_0$ ...
    On retrouve ce qu'on avait pour [L2] i.e. $\max \Delta f$ lorsque $p=2$?
\end{note}

\newpage

\section{Autre Méthode}

Pour $0\leq \varepsilon$,

\[ \left \{ \begin{array}{cc}
    -\alpha_\varepsilon\Delta u_\varepsilon + u_\varepsilon = f, & \text{dans}\ D, \\
    \partial_n u_\varepsilon = 0, & \text{sur}\ \partial D,
\end{array}
\right .\]

avec

\[ \alpha_\varepsilon = \begin{cases} 
    \alpha^1, & \text{dans}\ D\setminus B_\varepsilon, \\
    \alpha^0, & \text{dans}\ B_\varepsilon.
\end{cases} \]

La formulation variationnelle est : pour $\varphi$ dans $H^1(D)$,

\[ \int_D \alpha_\varepsilon\nabla u_\varepsilon\cdot\nabla\varphi\ dx + \int_D u_\varepsilon\varphi\ dx = \int_D f\varphi\ dx. \]

On pose alors 

\[ a_\varepsilon(u,\varphi) := \int_D \alpha_\varepsilon\nabla u\cdot\nabla\varphi\ dx + \int_D u\varphi\ dx, \]
\[ l_\varepsilon(\varphi) := \int_D f\varphi\ dx. \]

\subsection{Variations}

\subsubsection{Variations de la forme bilinéaire} 

\begin{proposition}
    \[ a_\varepsilon(u_0, v_\varepsilon) - a_0(u_0, v_\varepsilon) = \pi\varepsilon^2 (\alpha^0-\alpha^1)\nabla u_0(x_0)\cdot\nabla v_0(x_0) + O(\varepsilon^2). \]
\end{proposition}
\begin{proof}
    \[ a_\varepsilon(u_0, v_\varepsilon) - a_0(u_0, v_\varepsilon) = \int_D \alpha_\varepsilon\nabla u_0\cdot\nabla v_\varepsilon\ dx + \int_D u_0 v_\varepsilon\ dx - \int_D \alpha_0\nabla u_0\cdot\nabla v_\varepsilon\ dx - \int_D u_0 v_\varepsilon\ dx \]
    
    \[ = \int_{D\setminus B_\varepsilon} \alpha^1\nabla u_0\cdot\nabla v_\varepsilon\ dx + \int_{B_\varepsilon} \alpha^0\nabla u_0\cdot\nabla v_\varepsilon\ dx - \int_D \alpha^1\nabla u_0\cdot\nabla v_\varepsilon\ dx \]
    
    \[ = \int_{B_\varepsilon} (\alpha^0-\alpha^1)\nabla u_0\cdot\nabla v_\varepsilon\ dx \]
    
    \[ = \int_{B_\varepsilon} (\alpha^0-\alpha^1)\nabla u_0\cdot\nabla v_0\ dx + \int_{B_\varepsilon} (\alpha^0-\alpha^1)\nabla u_0\cdot\nabla (v_\varepsilon-v_0)\ dx \]
    
    Taylor : 
    
    \[ = \pi\varepsilon^2 (\alpha^0-\alpha^1)\nabla u_0(x_0)\cdot\nabla v_0(x_0) + \int_{B_\varepsilon} (\alpha^0-\alpha^1)\nabla u_0\cdot\nabla (v_\varepsilon-v_0)\ dx + O(\varepsilon^4) \]
\end{proof}

\subsubsection{Variations de la forme bilinéaire} 

\begin{proposition}
    \[ l_\varepsilon(v_\varepsilon) - l_0(v_\varepsilon) = 0. \]
\end{proposition}

\subsubsection{Variations de la fonction coût} 

\begin{proposition}
    \[ J_\varepsilon(v_\varepsilon) - J_\varepsilon(v_0) - DJ_\varepsilon(v_0)(v_\varepsilon - v_0) = f(\varepsilon)\delta J_1 + o\big( f(\varepsilon) \big), \]
\end{proposition}
\begin{proof}
    \[ DJ_\varepsilon(u_0)(u_\varepsilon - u_0) = \int |u_0-f|^{p-2} u_0(u_\varepsilon - u_0)\ dx \]
    
    D'où 
    
    \[ J_\varepsilon(u_\varepsilon) - J_\varepsilon(u_0) - DJ_\varepsilon(u_0)(u_\varepsilon - u_0) = \frac{1}{p}\int_D |u_\varepsilon - f|^p\ dx - \frac{1}{p}\int_D |u_0 - f|^p\ dx - \int |u_0-f|^{p-2} u_0(u_\varepsilon - u_0)\ dx \]
\end{proof}

\begin{proposition}
    \[ J_\varepsilon(u_0) - J_0(u_0) = 0. \]
\end{proposition}
