# Supplementary material for: Adjoint Method in PDE-based Image Compression
Source: arXiv:2302.02665 source file (2024-10-10)
Supplement: Supplementary file 9 [file appendix06.tex]

\section{En 1D}

\subsection{Solution sans trou}

\[ v_0^{g,\phi} = \lambda_0(x) e^{x/\sqrt{\alpha}} + \mu_0(x) e^{-x/\sqrt{\alpha}}. \]

\subsubsection{Si $g=0$}

\[ \lambda_0 = -\frac{e^{\frac{R}{\sqrt{\alpha}}} \phi\left(-R\right) - e^{\left(\frac{3 \, R}{\sqrt{\alpha}}\right)} \phi\left(R\right)}{e^{\left(\frac{4 \, R}{\sqrt{\alpha}}\right)} - 1}, \]

\[ \mu_0 = \frac{e^{\left(\frac{3 \, R}{\sqrt{\alpha}}\right)} \phi\left(-R\right) - e^{\frac{R}{\sqrt{\alpha}}} \phi\left(R\right)}{e^{\left(\frac{4 \, R}{\sqrt{\alpha}}\right)} - 1}. \]

\subsection{Solution avec trou}

\[ v_\varepsilon^{g,\phi} = \lambda_\varepsilon(x) e^{x/\sqrt{\alpha}} + \mu_\varepsilon(x) e^{-x/\sqrt{\alpha}}. \]

\subsubsection{Si $g=0$}

Sur $]\varepsilon,R[$ : 

\[ \lambda_\varepsilon^+ = \frac{e^{\frac{R}{\sqrt{\alpha}}} \phi\left(R\right)}{e^{\left(\frac{2 \, R}{\sqrt{\alpha}}\right)} - 1}, \]
\[ \mu_\varepsilon^+ = -\frac{e^{\frac{R}{\sqrt{\alpha}}} \phi\left(R\right)}{e^{\left(\frac{2 \, R}{\sqrt{\alpha}}\right)} - 1}. \]

Sur $]-R,-\varepsilon[$ : 

\[ \lambda_\varepsilon^- = -\frac{e^{\frac{R}{\sqrt{\alpha}}} \phi\left(-R\right)}{e^{\left(\frac{2 \, R}{\sqrt{\alpha}} + \frac{2 \, \epsilon}{\sqrt{\alpha}}\right)} - 1}, \]
\[ \mu_\varepsilon^- = \frac{e^{\left(\frac{R}{\sqrt{\alpha}} + \frac{2 \, \epsilon}{\sqrt{\alpha}}\right)} \phi\left(-R\right)}{e^{\left(\frac{2 \, R}{\sqrt{\alpha}} + \frac{2 \, \epsilon}{\sqrt{\alpha}}\right)} - 1}. \]

\subsection{Variation de $a$}

\[\int_{\partial B_R} \partial_n (v_\varepsilon^{0,v_0} - v_0^{0,v_0})\ d\sigma = \frac{1}{\sqrt{\alpha}}(\lambda_\varepsilon^+ - \lambda_0 - \mu_\varepsilon^- + \mu_0)e^{R/\sqrt{\alpha}}+\frac{1}{\sqrt{\alpha}}(\lambda_\varepsilon^- - \lambda_0 - \mu_\varepsilon^+ + \mu_0)e^{-R/\sqrt{\alpha}} \]

\[ = \frac{2 \, {\left(e^{\left(\frac{2 \, R}{\sqrt{\alpha}}\right)} v_0\left(-R\right) - e^{\left(\frac{2 \, R}{\sqrt{\alpha}} + \frac{2 \, \epsilon}{\sqrt{\alpha}}\right)} v_0\left(-R\right)\right)} \sqrt{\alpha}}{\alpha e^{\left(\frac{2 \, R}{\sqrt{\alpha}}\right)} - {\left(\alpha e^{\left(\frac{4 \, R}{\sqrt{\alpha}}\right)} - \alpha e^{\left(\frac{2 \, R}{\sqrt{\alpha}}\right)}\right)} e^{\left(\frac{2 \, \epsilon}{\sqrt{\alpha}}\right)} - \alpha} \]

\[ y(x) = K_{1} e^{\left(\frac{x}{\alpha^{\frac{1}{4}}}\right)} + K_{2} e^{\left(-\frac{x}{\alpha^{\frac{1}{4}}}\right)} - \frac{{\left(e^{\left(\frac{2 \, x}{\alpha^{\frac{1}{4}}}\right)} \int e^{\left(-\frac{x}{\alpha^{\frac{1}{4}}}\right)} g\left(x\right)\,{d x} - \int e^{\left(\frac{x}{\alpha^{\frac{1}{4}}}\right)} g\left(x\right)\,{d x}\right)} e^{\left(-\frac{x}{\alpha^{\frac{1}{4}}}\right)}}{2 \, \alpha^{\frac{1}{4}}} \]
