# Supplementary material for: Adjoint Method in PDE-based Image Compression
Source: arXiv:2302.02665 source file (2024-10-10)
Supplement: Supplementary file 20 [file appendix01.tex]

\section{Additional Proofs}
\label{appendix:properties-proofs}

Here, we give some proofs of results stated in the paper.

% \begin{proof}[Proof of Proposition \ref{prop:symmetric-continuous}] \textbullet ~ It is sufficient to prove that $\alpha\int_{\partial B_R} T_\varepsilon v\,\varphi\ d\sigma$ is symmetric :
%     \begin{align*}
%         \alpha\int_{\partial B_R} T_\varepsilon v\,\varphi\ d\sigma & = \alpha\int_{\partial B_R} \partial_n v_\varepsilon^{0,v}\,\varphi\ d\sigma \\
%         %
%         & = \alpha\int_{\partial B_R} \partial_n v_\varepsilon^{0,v}\,v_\varepsilon^{0,\varphi}\ d\sigma \\
%         %
%         & = \alpha\int_{B_R} \Delta v_\varepsilon^{0,v}\,v_\varepsilon^{0,\varphi}\ dx + \alpha\int_{B_R} \nabla v_\varepsilon^{0,v}\cdot\nabla v_\varepsilon^{0,\varphi}\ dx \\
%         %
%         & = \int_{B_R} v_\varepsilon^{0,v}\,v_\varepsilon^{0,\varphi}\ dx + \alpha\int_{B_R} \nabla v_\varepsilon^{0,v}\cdot\nabla v_\varepsilon^{0,\varphi}\ dx.
%     \end{align*}
    
%     \textbullet ~ Let $\phi$ be in $H^{1/2}(\partial B_R)$,
%     \begin{align*}
%         \alpha\int_{\partial B_R} h_\varepsilon\, \phi\ d\sigma & = -\alpha\int_{\partial B_R} \partial_n v_\varepsilon^{h,0}\, v_\varepsilon^{0,\phi}\ d\sigma \\
%         %
%         & = -\alpha\int_{B_R}\Delta v_\varepsilon^{h,0}\,v_\varepsilon^{0,\phi}\ dx - \alpha\int_{B_R}\nabla v_\varepsilon^{h,0}\cdot\nabla v_\varepsilon^{0,\phi}\ dx \\
%         %
%         & = \int_{B_R} h\,v_\varepsilon^{0,\phi}\ dx - \int_{B_R} v_\varepsilon^{h,0}\,v_\varepsilon^{0,\phi}\ dx - \alpha\int_{B_R}\nabla v_\varepsilon^{h,0}\cdot\nabla v_\varepsilon^{0,\phi}\ dx \\
%         %
%         & = \int_{B_R} h\,v_\varepsilon^{0,\phi}\ dx - \int_{B_R} v_\varepsilon^{h,0}\,v_\varepsilon^{0,\phi}\ dx + \alpha\int_{B_R} v_\varepsilon^{h,0}\Delta v_\varepsilon^{0,\phi}\ dx - \alpha\int_{\partial B_R} \partial_n v_\varepsilon^{0,\phi}\,v_\varepsilon^{h,0}\ d\sigma \\
%         %
%         & = \int_{B_R} h\,v_\varepsilon^{0,\phi}\ dx + \alpha\int_{B_R} \underbrace{(\alpha\Delta v_\varepsilon^{0,\phi} - v_\varepsilon^{0,\phi})}_{=0}\,v_\varepsilon^{h,0}\ dx - \alpha\int_{\partial B_R} \partial_n v_\varepsilon^{0,\phi}\,\underbrace{v_\varepsilon^{h,0}}_{=0}\ d\sigma \\
%         %
%         & = \int_{B_R} h\,v_\varepsilon^{0,\phi}\ dx.
%     \end{align*}
% \end{proof}

% \begin{proof}[Proof of Proposition \ref{prop:w0-wD}]
%     We set $w_R := \widetilde{w}_0|_{D\setminus B_R}$. We have to show that $w_R=w_0$ i.e. $a_0(w_R,\varphi_R) = -DJ_0(v_0)\varphi_R$, $\forall \varphi_R\in V_R$. Let $\varphi_R\in V_R$. We denote $\widetilde{\varphi}\in V_0$ the extension of $\varphi_R$ to $V_0$ such that $-\alpha\Delta\widetilde{\varphi} + \widetilde{\varphi} = 0$ in $B_R$. Thus,
%     % Soit $\varphi\in H^1_0(D)$ telle que $-\alpha\Delta\varphi + \varphi = 0$ sur $B_R$. On pose $\varphi_R := \varphi|_{D\setminus B_R}$.
%     \begin{align*}
%         a_0(w_R,\varphi_R) & = \alpha\int_{D\setminus B_R}\nabla w_R\cdot\nabla\varphi_R\ dx + \alpha\int_{\partial B_R} T_0 w_R\, \varphi_R\ d\sigma + \int_{D\setminus B_R} w_R\,\varphi_R\ dx \\
%         %
%         & = \alpha\int_{D\setminus B_R}\nabla w_R\cdot\nabla\varphi_R\ dx + \alpha\int_{\partial B_R} T_0 w_R\, \varphi_R\ d\sigma + \int_{D\setminus B_R} w_R\,\varphi_R\ dx + \int_{B_R}\underbrace{(-\alpha\Delta\widetilde{\varphi} + \widetilde{\varphi})}_{=0} \widetilde{w}_0\ dx \\
%         %
%         & = \alpha\int_{D\setminus B_R}\nabla w_R\cdot\nabla\varphi_R\ dx + \alpha\int_{\partial B_R} T_0 w_R\, \varphi_R\ d\sigma + \int_{D\setminus B_R} w_R\,\varphi_R\ dx -\alpha \int_{B_R}\Delta\widetilde{\varphi} \widetilde{w}_0\ dx \\ & \hspace{3cm} + \int_{B_R}\widetilde{\varphi}\,\widetilde{w}_0\ dx \\
%         %
%         & = \alpha\int_{D\setminus B_R}\nabla w_R\cdot\nabla\varphi_R\ dx + \alpha\int_{\partial B_R} T_0 \varphi_R\,w_R\ d\sigma + \int_{D\setminus B_R} w_R\,\varphi\ dx + \alpha\int_{B_R}\nabla\widetilde{\varphi}\cdot\nabla \widetilde{w}_0\ dx \\ & \hspace{3cm} - \alpha\int_{\partial B_R}\partial_n \widetilde{\varphi}\, \widetilde{w}_0\ d\sigma + \int_{B_R}\widetilde{\varphi}\,\widetilde{w}_0\ dx \\
%         %
%         & = \alpha\int_{D\setminus B_R}\nabla w_R\cdot\nabla\varphi_R\ dx + \alpha\int_{\partial B_R} T_0 \varphi_R\,w_R\ d\sigma + \int_{D\setminus B_R} w_R\varphi_R\ dx + \alpha\int_{B_R}\nabla\widetilde{\varphi}\cdot\nabla \widetilde{w}_0\ dx \\ & \hspace{3cm} - \alpha\int_{\partial B_R}T_0 \varphi_R\, w_R\ d\sigma + \int_{B_R}\widetilde{\varphi}\,\widetilde{w}_0\ dx \\
%         %
%         & = \alpha\int_{D\setminus B_R}\nabla w_R\cdot\nabla\varphi_R\ dx + \int_{D\setminus B_R} w_R\varphi_R\ dx + \alpha\int_{B_R}\nabla\widetilde{\varphi}\cdot\nabla \widetilde{w}_0\ dx + \int_{B_R}\widetilde{\varphi}\,\widetilde{w}_0\ dx \\
%         %
%         & = \alpha\int_{D}\nabla \widetilde{w}_0\cdot\nabla\widetilde{\varphi}\ dx + \int_{D}\widetilde{w}_0\,\widetilde{\varphi}\ dx \\
%         %
%         & = \widetilde{a}_0(\widetilde{w}_0,\widetilde{\varphi}) = -D\widetilde{J}_0(v_D)\widetilde{\varphi}.
%     \end{align*}
%     Moreover, by definition $\widetilde{J}_0(v_D) = J_0(v_R)$, % pour tout $v\in V_0$ telle que $-\alpha\Delta v + v = \alpha\Delta f$ dans $B_R$ (on pose $v_R := v|_{D\setminus B_R}$). Et
%     thus, 
%     \[ D\widetilde{J}_0(v_D)\widetilde{\varphi} = DJ_0(v_0)\varphi_R. \]
%     % d'où,
%     % Enfin, soit $\varphi_R\in V_R$. On note $\varphi\in V_0$ l'extension de $\varphi_R$ à $V_0$ telle que $-\alpha\Delta\varphi + \varphi = 0$ dans $B_R$. Alors,
%     % \[ a_0(\varphi_R, w_R) = -DJ_0(v_0)\varphi_R. \]
%     By uniqueness of the solution, $w_R = w_0$.
% \end{proof}
